# Supplementary material for: XScale-NVS: Cross-Scale Novel View Synthesis with Hash Featurized Manifold
Source: arXiv:2403.19517 source file (2024-03-28)
Supplement: Supplementary file 1 [file X_suppl.tex]

\clearpage
\setcounter{page}{1}
\maketitlesupplementary

\section{Additional Dataset Details}
\begin{table}[htbp]
\scriptsize
\setlength{\tabcolsep}{3.2mm}{
\footnotesize
\begin{tabular}{cccc}
\hline
{Scene} & Area ($m^2$) & \#Images & Resolution \\ \hline
TW-Pavilion (Day) & $1.3\times 10^4$ & 10,999 & 5K/8K \\ 
TW-Pavilion (Night) & $1.3\times 10^4$ & 1,687 & 5K/8K \\ 
Lanes \& Alleys & $4.5\times 10^5$ & 18,206 & 5K/8K \\ 
The Great Wall (T3) & $3\times 10^6$ & 7,441 & 5K/8K \\ 
The Great Wall (T2) & $2\times 10^6$ & 6,372 & 5K/8K \\ 
The Five Old Peaks & $1.5\times 10^6$ & 3,960 & 5K/8K \\ 
Sandie Spring & $3\times 10^6$ & 5,474 & 5K/8K \\ 
\hline
\end{tabular}
}
\vspace{-1em}
\caption{Statistics of the \texttt{GigaNVS} dataset.}\label{tab:dataset}
\vspace{-1em}
\end{table}
Our dataset is captured using two drones and a handheld DSLR. The drones we use include a DJI Matrice 300 RTK equipped with a fixed 35mm camera, whose FOV is 63.5$^\circ$ and the image resolution is 5460$\times$8192. The other drone is a DJI Mavic 3 mounted with a fixed 24mm camera, whose FOV is 84$^\circ$ and the image resolution is 3956$\times$5280. The ground photography is captured by a Canon EOS R5 DSLR camera with a 15-30mm lens, and the image resolution is 5464$\times$8192. Since we focus on in-the-wild ultra-large-scale scenes and aim to collect high-quality multi-view imagery of varying scales, it is difficult to finish capturing within a short period to maintain a constant illumination condition. We therefore manually adjust the ISO, white balance, shutter speed, and aperture size of the cameras according to the illumination condition to prioritize the imaging quality.

A detailed statistics of our dataset is listed in Table~\ref{tab:dataset}. The scenes we capture typically span areas of several square kilometers. For each scene, we capture between 1,687 and 18,206 images taking several days. We use shared intrinsic parameters for images captured from the same camera, and we use Agisoft Metashape~\cite{agisoft} to compute the camera poses, undistort the images, and reconstruct the mesh. We take every 7th photo as our test set for each scene, which approximates a uniform coverage of all view points and scales. 

\section{Additional Implementation Details}
In this section, we further detail the implementations of our model and the training strategies we use, and then present details regarding the comparative evaluations.
\par\noindent\textbf{Additional Model Details.}
We use $L=16$ levels of multi-resolution hash encoding with a coarsest resolution of 16 and a finest resolution of $2^{13}\sim2^{19}$ depending on the scene scale and the image resolution. We use a maximum number of $N_h=2^{22}$ hash entries with $Z=8$ feature channels, following~\cite{li2023neuralangelo}. The mesh is reconstructed using Agisoft Metashape~\cite{agisoft} and we set the multisampling rate $\gamma$ as 2 during rasterization. The only loss function we use is the L1 photometric error. The decoder MLP $\mathcal{M}$ and the manifold {deformation MLP $\xi$} consist of 4 and 2 layers respectively, where each layer contains 64 hidden units. The concatenated multi-resolution hash features are consumed through FiLM-conditioning~\cite{perez2018film, chan2021pi}. To compensate for the camera response variations of the real-world captures, we follow~\cite{barron2023zip, li2023neuralangelo} to use appearance embedding to modulate the intermediate features of the decoder $\mathcal{M}$. 

\par\noindent\textbf{Additional Training Details.} 
To enable a large batch size of camera views during training, we pre-cache the rasterized z-buffer of the reconstructed mesh for each training view. At each training iteration, we sample a random set of camera views and then a random batch of pixel rays from the caches for each sampled view. We use a batch size of 16 for the random views and a batch size of 16384 for the random rays. We train our model using the Adam optimizer~\cite{kingma2014adam} with a learning rate of $10^{-4}$ for 1000 epochs, randomly iterating through all training views to complete a single epoch. 
% where the L1 loss between the rendered colour and the observed pixel colour is minimized. 
The training can be done with a single NVIDIA RTX3090 GPU. 
% \guangyu{\#Images per scene we select for the experiments}
\par\noindent\textbf{Additional Evaluation Details.} Similar to \cite{10274871}, we only focus on the reconstruction of foreground regions. For a fair comparison to other baselines~\cite{kerbl20233d, muller2022instant, li2023neuralangelo}, we leverage the mesh to explicitly benefit their performance by providing not only the geometric guidance but also foreground mask priors. Specifically, we project the mesh to fill the background regions of all input images as pure white, i.e., $[255,255,255]$,  and set the background colour in \cite{kerbl20233d, muller2022instant, li2023neuralangelo} explicitly as the same white colour during training. We find this simple modification effectively bypasses the difficult background modelling task and significantly boosts the foreground rendering quality of these methods. 
% \guangyu{add iNGP visual comparisons with and without white bg.} 
We also use the rasterized foreground mask to calculate an additional BCE loss as done in~\cite{wang2021neus} to further regularize the foreground geometry of \cite{kerbl20233d, muller2022instant, li2023neuralangelo}. Before computing the evaluation metrics, we apply the same rasterized mask to the renderings of all competing methods and the corresponding ground truth image. We fairly evaluate our method and all other baselines using the same NVIDIA RTX3090 GPU. 

\begin{figure*}[htbp]
    \centering
    
    \newcommand{\figw}{1.0} % can bigger than 1
    \includegraphics[width=\figw\textwidth,trim={0cm 0cm 0cm 0cm},clip]{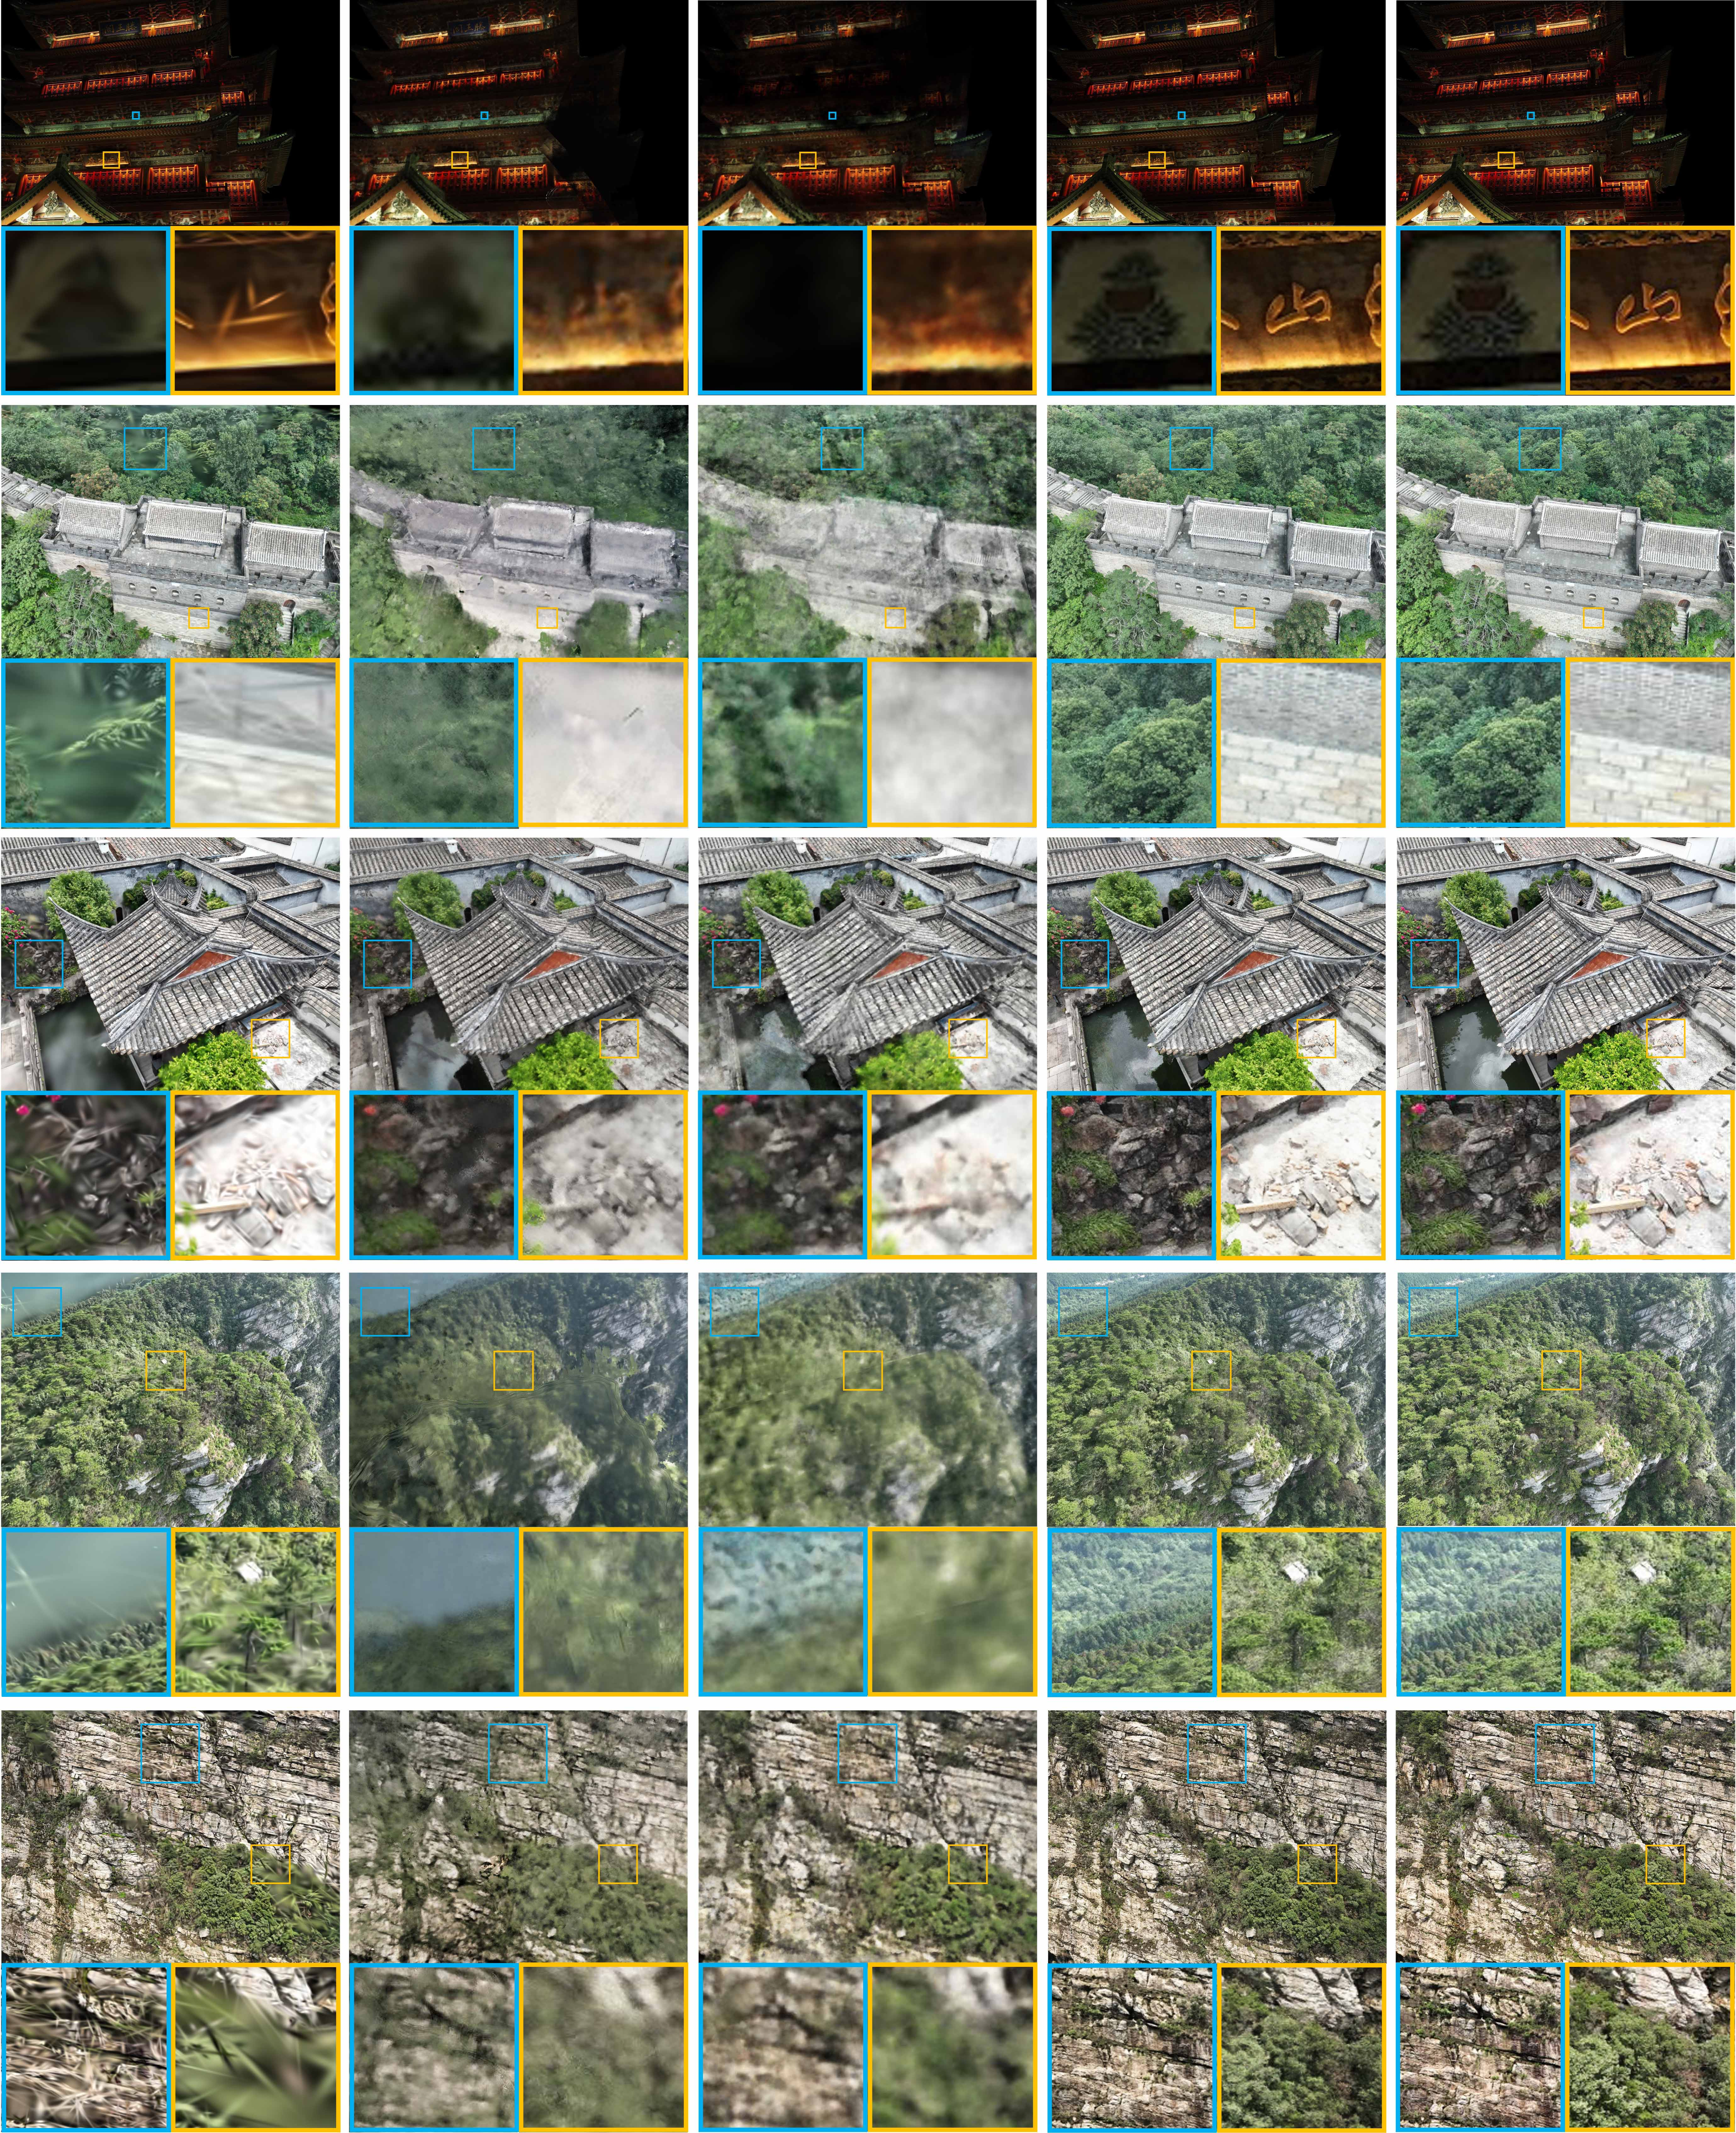}
\hfill
\vspace{-1.5em}
\centerline{\footnotesize{\hspace{-1.5em}
    (a) 3D Gaussian Splatting~\cite{kerbl20233d}\hspace{2.0em}(b) Neuralangelo~\cite{li2023neuralangelo}\hspace{5.0em}(c) iNGP~\cite{muller2022instant}\hspace{8.0em}(d) \textbf{Ours}\hspace{5.5em}
    (e) Ground Truth Image}}
\vspace{-1.5em}
\caption{Qualitative comparisons of 1K-resolution novel view synthesis on the \texttt{GigaNVS} dataset. Compared to \cite{muller2022instant, kerbl20233d, li2023neuralangelo}, our hash featurized manifold represents cross-scale contents with superior fidelity and effectively preserves the rich details of the original imagery.}
\label{fig:qualitative_supp}
\end{figure*}
\begin{figure*}[htb]
    %\centering
    %\centering
    
    \newcommand{\figw}{1.0} % can bigger than 1
    %\begin{minipage}{\colw\linewidth}
    \vspace{-1em}
    \centering
    \includegraphics[width=\figw\textwidth,trim={0cm 0cm 0cm 0cm},clip]{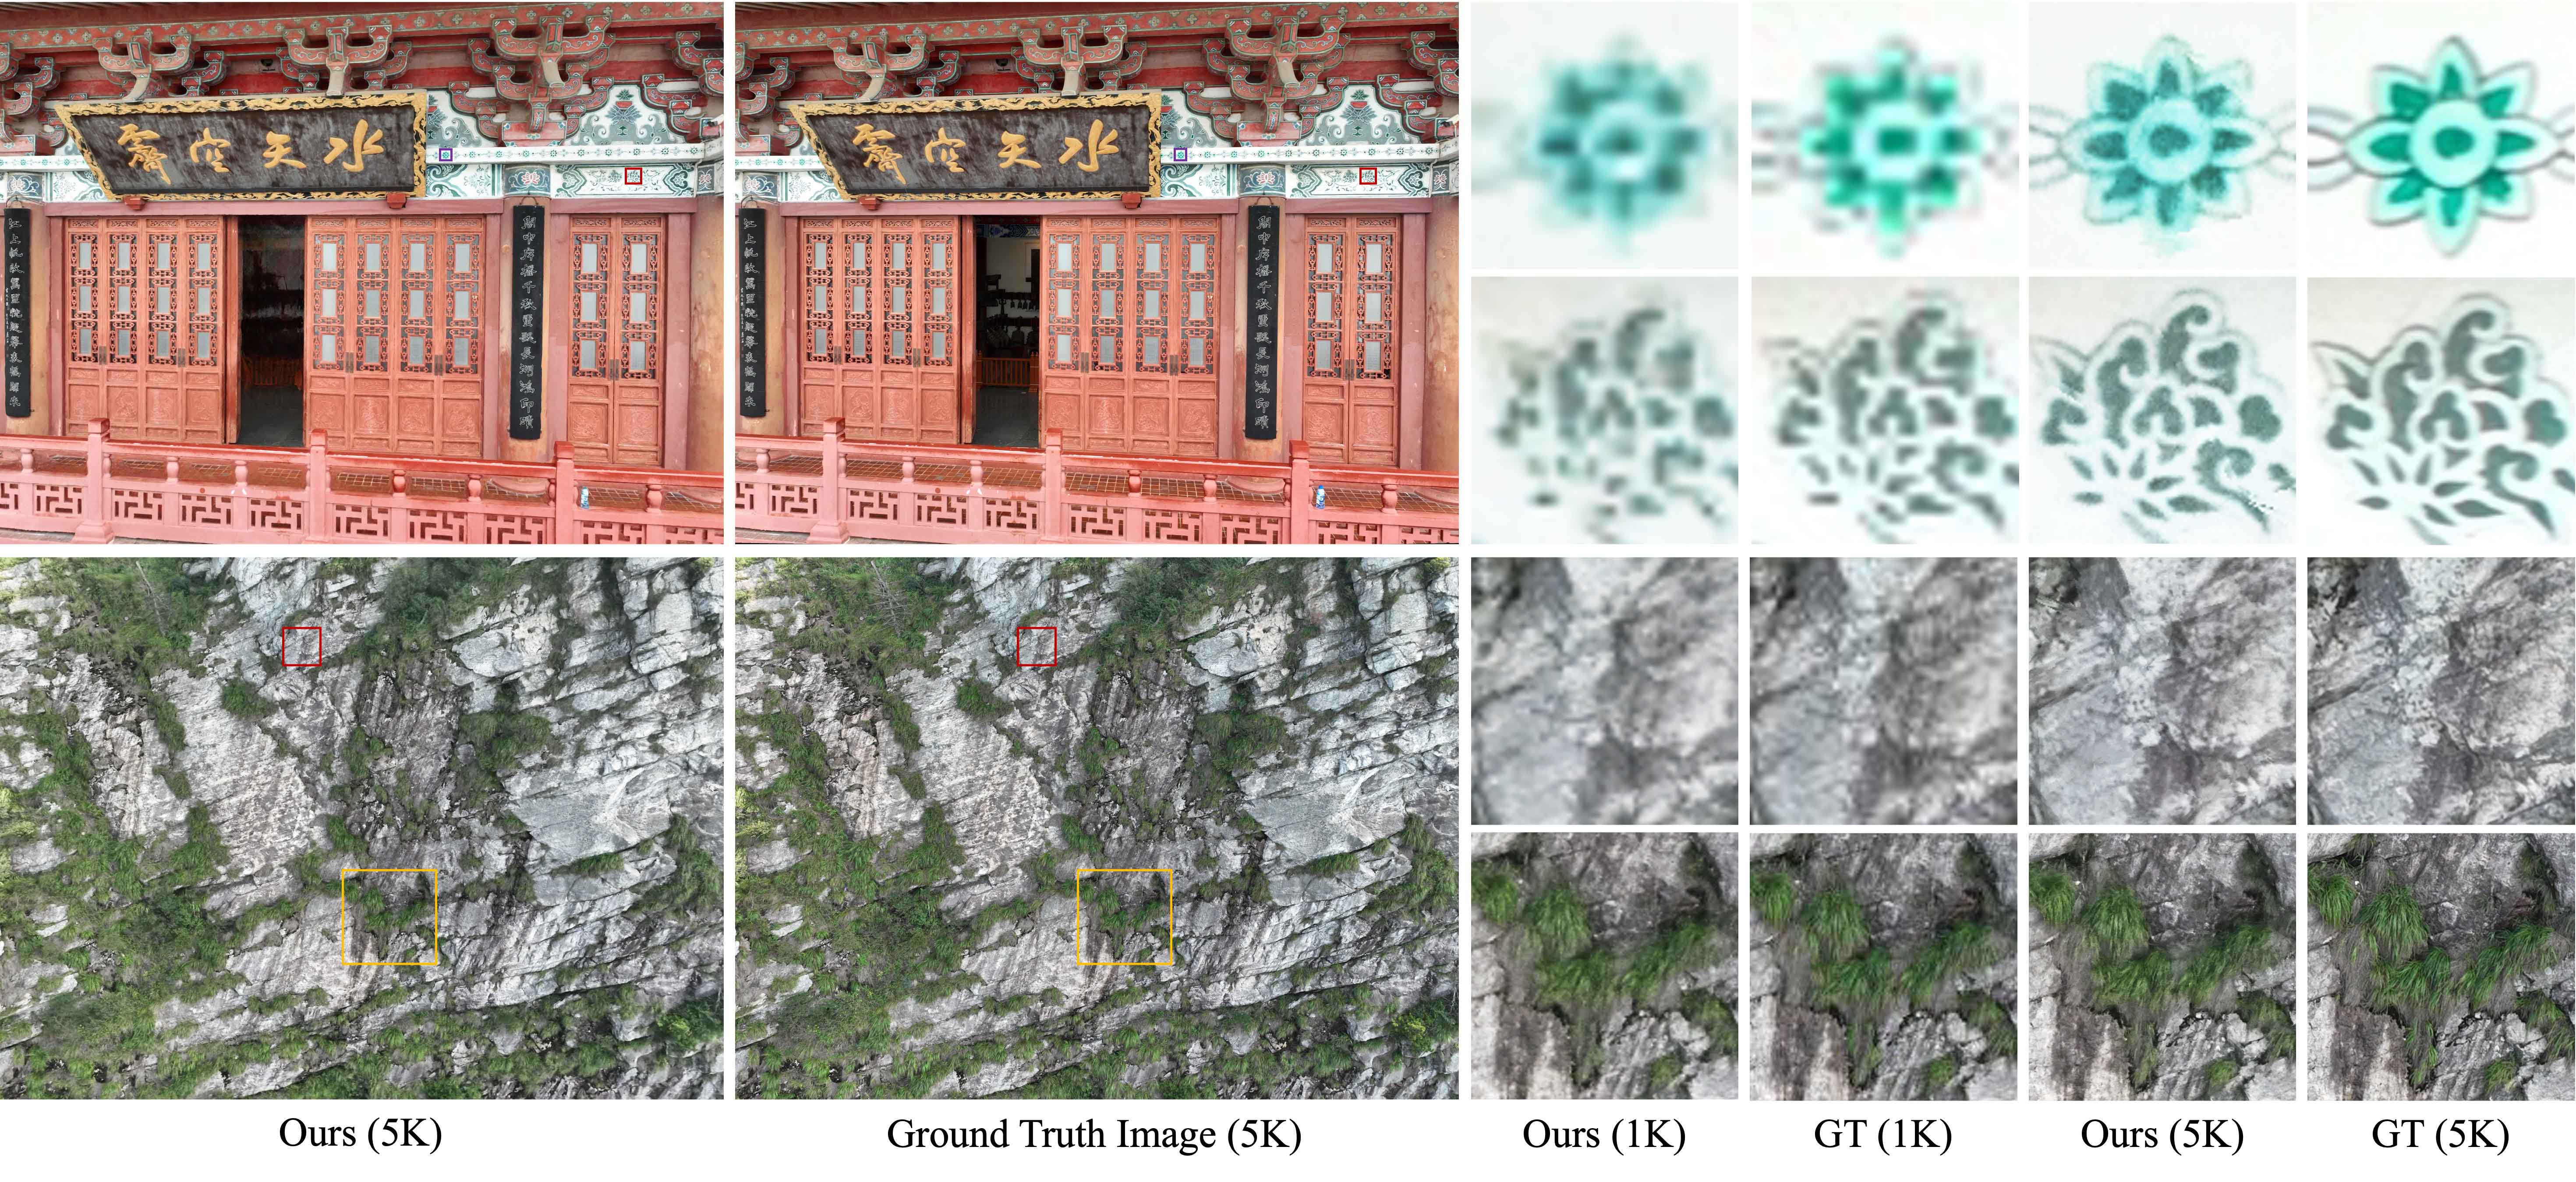}
    \vspace{-2.2em}
    \caption{Qualitative results of 5K-resolution novel view synthesis on the \texttt{GigaNVS} dataset. Our method fully exploits the input resolution and demonstrates strong scalability towards high-resolution neural rendering. Please zoom-in to see the high-resolution details.}
    \hfill
    % \vspace{-1.0em}
    \label{fig:qualitative_6k}
\end{figure*}
\begin{figure*}[htbp]
    \centering
    
    \newcommand{\figw}{1.0} % can bigger than 1
    \includegraphics[width=\figw\textwidth,trim={0cm 0cm 0cm 0cm},clip]{}
\hfill
\vspace{-1.5em}
\centerline{\footnotesize{\hspace{-1.5em}
    (a) 3D Gaussian Splatting~\cite{kerbl20233d}\hspace{2.0em}(b) Neuralangelo~\cite{li2023neuralangelo}\hspace{5.0em}
    (c) iNGP~\cite{muller2022instant}\hspace{8.0em}(d) \textbf{Ours}\hspace{6.0em}
    (e) Ground Truth Image}}
\vspace{-1.5em}
\caption{Visual comparisons on the Tanks\&Temples dataset~\cite{knapitsch2017tanks}. Our method excels at recovering local intricate details yet generally performs on par with state-of-the-art neural rendering methods~\cite{kerbl20233d, muller2022instant, li2023neuralangelo} on small-scale scenes.}
\vspace{-0.5em}
\label{fig:qualitative_tanks}
\end{figure*}
% Please add the following required packages to your document preamble:
% \usepackage{multirow}
\begin{table*}[htbp]
\centering
\newcommand{\tabincell}[2]{\begin{tabular}{@{}#1@{}}#2\end{tabular}}
\footnotesize
\setlength{\tabcolsep}{0.55mm}{
% \caption{Quantitative comparisons at 1K (989$\times$ 1320) resolution on GigaNVS dataset. The proposed hash featurized manifold outperforms state-of-the-art approaches on all evaluation metrics.}
% \vspace{-1em}
\begin{tabular}{c|ccc|ccc|ccc|ccc|ccc}
\hline
\multirow{2}{*}{\tabincell{c}{Scene}} & \multicolumn{3}{c|}{Meta representation\cite{10274871}} & \multicolumn{3}{c|}{3D Gaussian Splatting\cite{kerbl20233d}} & \multicolumn{3}{c|}{Neuralangelo\cite{li2023neuralangelo}} & \multicolumn{3}{c|}{iNGP\cite{muller2022instant}} & \multicolumn{3}{c}{\textbf{Ours}} \\ \cline{2-16}
{} & PSNR $\uparrow$ & SSIM $\uparrow$ & LPIPS$\downarrow$ & PSNR $\uparrow$ & SSIM $\uparrow$ & LPIPS$\downarrow$ & PSNR $\uparrow$ & SSIM $\uparrow$ & LPIPS$\downarrow$ & PSNR $\uparrow$ & SSIM $\uparrow$ & LPIPS$\downarrow$ & PSNR $\uparrow$ & SSIM $\uparrow$ & LPIPS$\downarrow$\\ \hline
Family & 27.92 & 0.913 & \cellcolor{Third}0.035 & \cellcolor{First}{28.54} & \cellcolor{Second}0.920 & \cellcolor{Third}0.035 & 28.02 & \cellcolor{First}{0.922} & \cellcolor{Second}0.033 & \cellcolor{Second}{28.49} & \cellcolor{Third}{0.919} & {0.036} & \cellcolor{Third}{28.15} & {0.915} & \cellcolor{First}{0.032} \\
Francis & \cellcolor{Third}33.11 & \cellcolor{Third}0.958 & \cellcolor{Second}0.048 & \cellcolor{First}{35.77} & \cellcolor{Second}0.969 & \cellcolor{Third}0.050 & 30.54 & 0.951 & 0.056 & {31.85} & {0.950} & {0.067} & \cellcolor{Second}35.32 & \cellcolor{First}{0.973} & \cellcolor{First}{0.024} \\
Horse & \cellcolor{Second}35.22 & \cellcolor{Third}0.979 & 0.027 & 34.88 & \cellcolor{First}{0.986} & \cellcolor{Second}0.017 & 34.62 & \cellcolor{Second}0.984 & \cellcolor{First}{0.016} & \cellcolor{Third}{35.16} & \cellcolor{Second}{0.984} & \cellcolor{Third}{0.018} & \cellcolor{First}{36.07} & \cellcolor{Second}0.984 & \cellcolor{Second}0.017 \\
M60 & 27.36 & 0.891 & 0.153 & \cellcolor{First}{29.41} & \cellcolor{First}{0.918} & \cellcolor{Third}0.133 & 27.03 & 0.886 & 0.154 & \cellcolor{Second}{28.82} & \cellcolor{Second}{0.907} & \cellcolor{Second}{0.132} & \cellcolor{Third}28.07 & \cellcolor{Third}0.899 & \cellcolor{First}{0.115} \\
Lighthouse & 23.92 & 0.811 & 0.201 & 22.49 & 0.825 & 0.207 & \cellcolor{Third}23.96 & \cellcolor{Third}{0.836} & \cellcolor{Third}0.191 & \cellcolor{Second}{24.47} & \cellcolor{Second}{0.842} & \cellcolor{Second}{0.187} & \cellcolor{First}{26.47} & \cellcolor{First}{0.866} & \cellcolor{First}{0.127} \\
Panther & \cellcolor{Third}28.57 & 0.889 & 0.162 & 26.83 & 0.869 & 0.210 & 27.87 & \cellcolor{Third}0.901 & \cellcolor{Third}0.155 & \cellcolor{First}{29.70} & \cellcolor{First}{0.908} & \cellcolor{Second}{0.146} & \cellcolor{Second}{29.05} & \cellcolor{Second}{0.903} & \cellcolor{First}{0.112} \\
Train & 22.12 & 0.803 & 0.207 & \cellcolor{Second}22.44 & \cellcolor{Second}0.834 & 0.206 & 19.85 & 0.806 & \cellcolor{Third}0.195 & \cellcolor{Third}{22.21} & \cellcolor{Third}{0.826} & \cellcolor{Second}{0.184} & \cellcolor{First}{24.50} & \cellcolor{First}{0.863} & \cellcolor{First}{0.124} \\ \hline
Mean & 28.32 & 0.892 & 0.119 & \cellcolor{Third}28.62 & \cellcolor{Third}0.903 & 0.123 & 27.41 & 0.898 & \cellcolor{Third}0.114 & \cellcolor{Second}{28.67} & \cellcolor{Second}{0.905} & \cellcolor{Second}{0.110} & \cellcolor{First}29.66 & \cellcolor{First}0.914 & \cellcolor{First}0.079 \\ \hline
\end{tabular}
}
\vspace{-1em}
\caption{Quantitative comparisons on seven scenes from the Tanks\&Temples dataset. 
% Our method also outperforms state-of-the-art approaches on small-scale scenes.
}
\label{tab:tanks}
\vspace{1.0em}
\end{table*}
\begin{figure*}[htb]
    %\centering
    %\centering
    
    \newcommand{\figw}{1.0} % can bigger than 1
    %\begin{minipage}{\colw\linewidth}
    \vspace{-1em}
    \centering
    \includegraphics[width=\figw\textwidth,trim={0cm 0cm 0cm 0cm},clip]{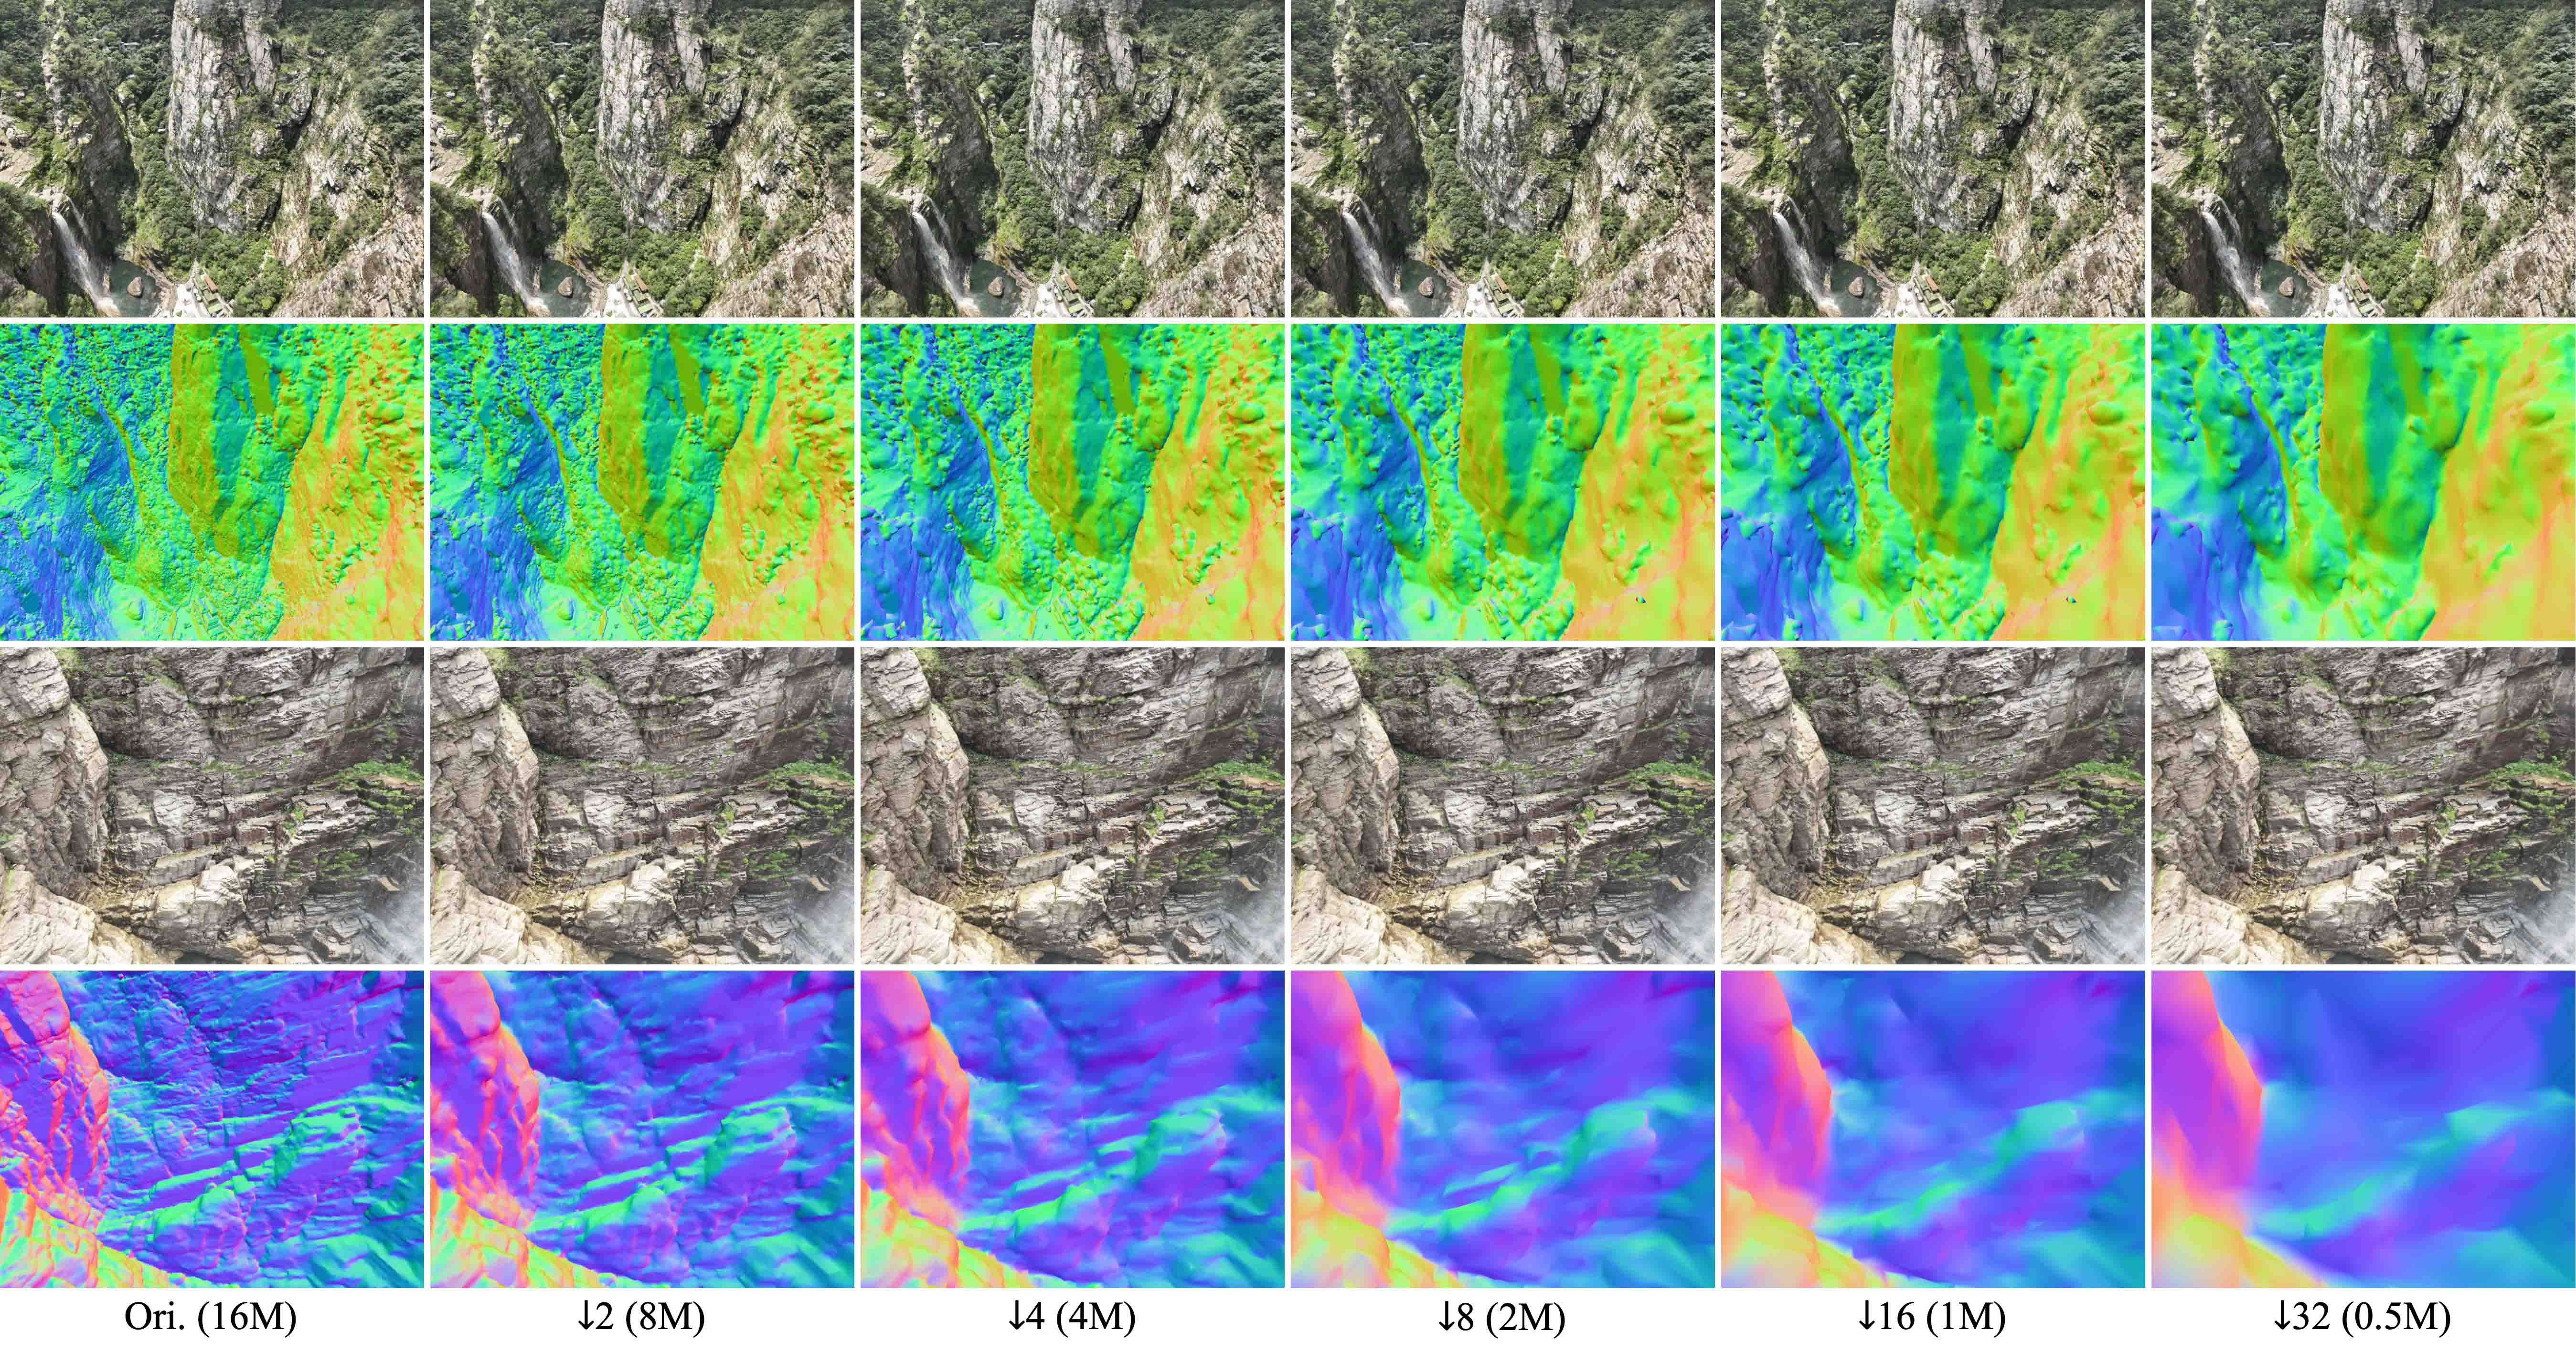}
    \vspace{-2.2em}
    \caption{Qualitative results with different mesh resolutions on the Sandie Spring scene of \texttt{GigaNVS} dataset, where our novel view RGB renderings and the corresponding mesh normals are visualized. The first two rows are macro-scale renderings from a distance and the last two rows are micro-scale renderings at the close-up. Our method robustly recovers scene contents at drastically different scales when down-sampling the mesh to lower resolutions.}
    \hfill
    \vspace{-1.5em}
    \label{fig:qualitative_mesh}
\end{figure*}
\begin{figure*}[htbp]
    %\centering
    %\centering
    
    \newcommand{\figw}{1.0} % can bigger than 1
    %\begin{minipage}{\colw\linewidth}
    % \vspace{-1em}
    \centering
    \includegraphics[width=\figw\textwidth,trim={0cm 0cm 0cm 0cm},clip]{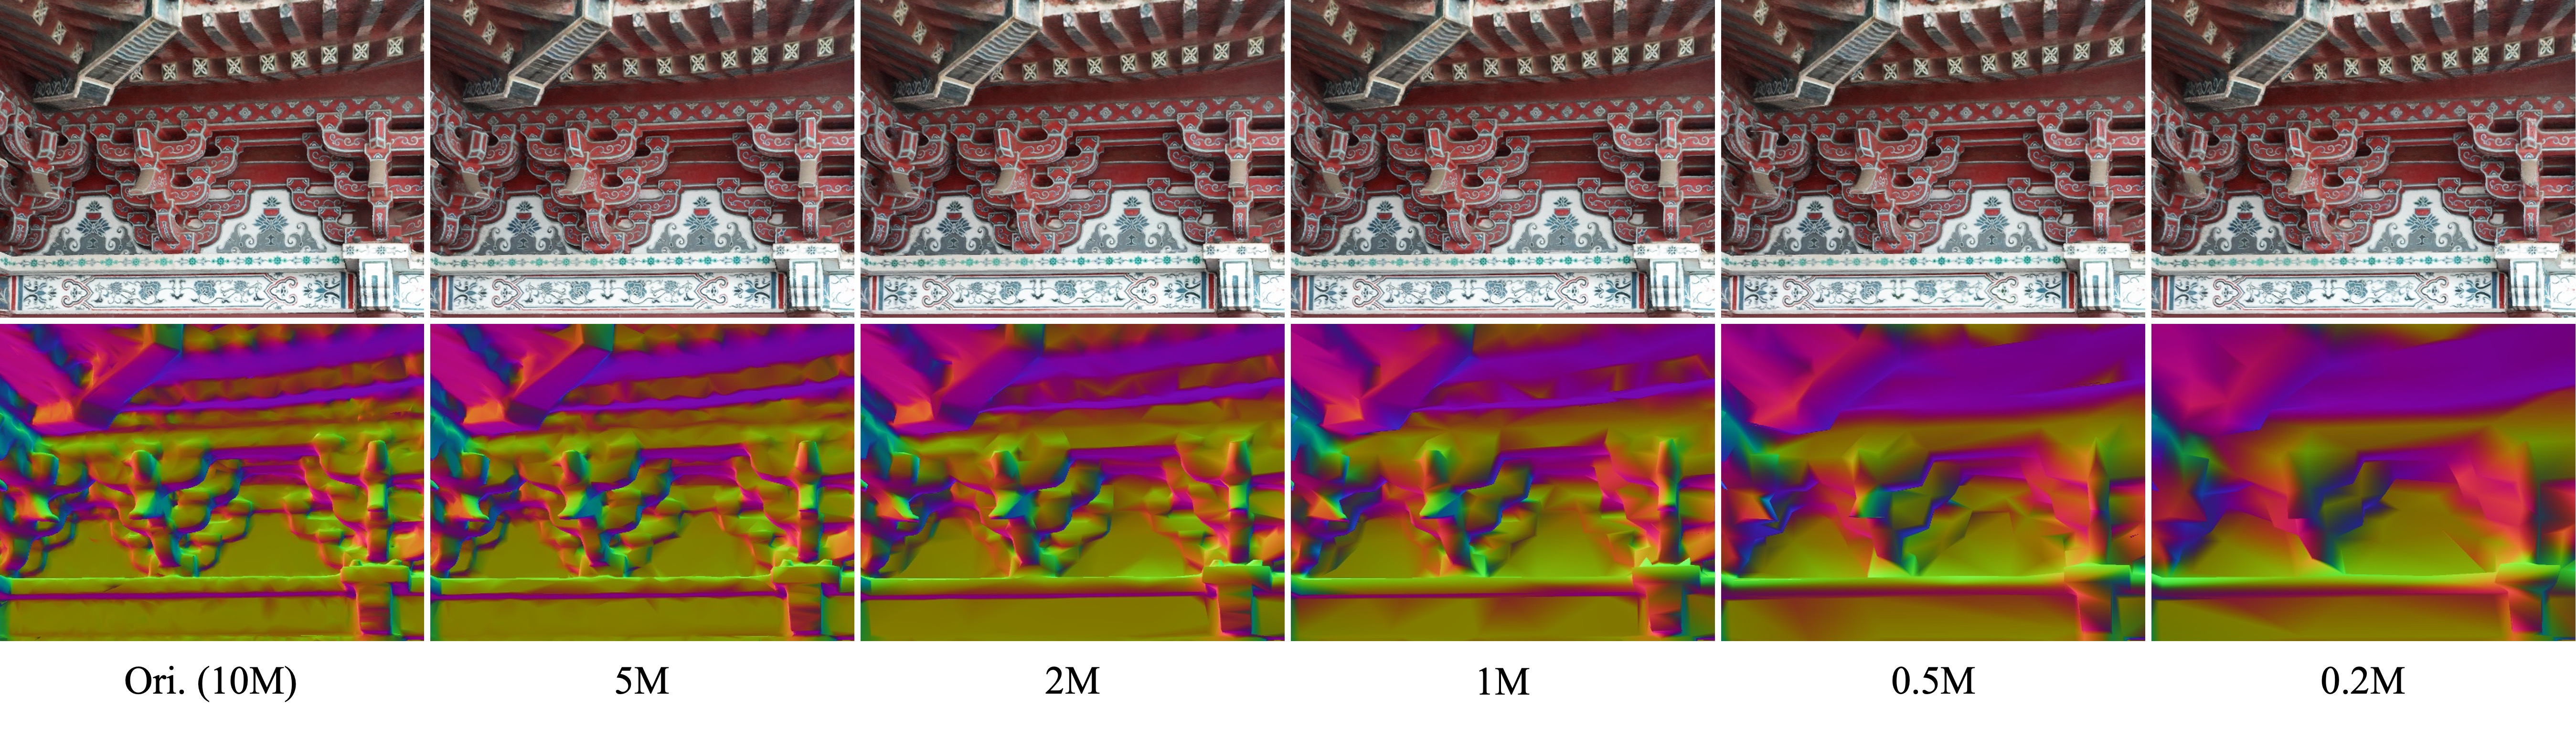}
    \vspace{-2.2em}
    \caption{Qualitative results with different mesh resolutions on the TW-Pavilion (Day) scene of \texttt{GigaNVS} dataset. First row: our novel view RGB renderings; Second row: the corresponding rendered normals of the input mesh. }
    \hfill
    \vspace{-1.5em}
    \label{fig:qualitative_mesh_twg}
\end{figure*}

\section{Additional Results on \textbf{\texttt{GigaNVS}}}
In this section, we present additional qualitative results on the challenging \texttt{GigaNVS} dataset. 
\par\noindent\textbf{1K-resolution Novel View Synthesis.}
We first compare against prior state-of-the-art approaches~\cite{muller2022instant, kerbl20233d, li2023neuralangelo} on novel view synthesis with 1K resolution images as inputs and outputs. The corresponding qualitative results are shown in Fig.~\ref{fig:qualitative_supp}. Our hash featurized manifold synthesizes novel views with significantly superior fidelity compared to other baselines, effectively recovering realistic cross-scale details of the relievos, plants, tiles, and stones, reflecting unprecedentedly rich contents in real-world large-scale scenes. 

\par\noindent\textbf{5K-resolution Novel View Synthesis.}
To take a step further, our method can operate effectively on high-resolution inputs of 5K or 8K due to the expressivity and efficiency, whereas existing baselines are not scalable towards this high-resolution setup, since they still struggle to render the details at 1K resolution (see Fig.~\ref{fig:qualitative_supp} (a), (b), (c)) and suffer from memory issues. In Fig.~\ref{fig:qualitative_6k}, we provide our 5K novel view synthesis results where our model is trained using the original 5K resolution imagery. The results suggest that our method can successfully exploit the rich information brought by the high-resolution imagery and represent scenes using approximately the input-level resolution. As observed, our 5K rendering delivers significantly richer details compared to the ground truth image of 1K resolution, indicating a continuously better perceptual quality proportional to the input resolution, which hash rarely been verified in existing in-the-wild neural rendering methods. Therefore, the proposed hash featurized manifold representation shows great potential to bridge the resolution gap between sensation and reconstruction. 

\section{Additional Results on Tanks\&Temples}
We now present more detailed results on the public Tanks\&Temples dataset~\cite{knapitsch2017tanks}. Following~\cite{10274871}, we select seven real-world outdoor scenes from this dataset to benchmark our performance on small-scale scenarios. In Fig.~\ref{fig:qualitative_tanks}, we show visual comparisons of the competing methods on four representative scenes. In general, our method performs on par with state-of-the-art baselines~\cite{kerbl20233d, muller2022instant, li2023neuralangelo} while only showing slight improvements at fine-grained details, with the micro-scale intricate textures on the sculpture and tanks better recovered. The quantitative evaluations are reported in Table~\ref{tab:tanks}. Our method yields a $\sim$1dB improvement in PSNR and a 28\% lower LPIPS relative to the second best method iNGP~\cite{muller2022instant}. Therefore, hash featurized manifold can serve as a general purpose neural scene representation offering superior expressivity and efficiency.

\section{Additional Ablations}
In this section, we provide additional ablations to conduct a more comprehensive demonstration of our design. 
\label{supp:ablation}
\par\noindent\textbf{Featurization Enhancements.}
The surface multisampling and manifold deformation serve as optional enhancements upon the hash featurized manifold representation, which can help to better describe the cross-scale scene details. As shown in Fig.~\ref{fig:ablation_md}, our method can subsequently render sharper details after introducing these designs. 
\begin{figure}[htb]
    %\centering
    %\centering
    
    \newcommand{\figw}{0.48} % can bigger than 1
    %\begin{minipage}{\colw\linewidth}
    % \vspace{-1em}
    \centering
    \includegraphics[width=\figw\textwidth,trim={0cm 0cm 0cm 0cm},clip]{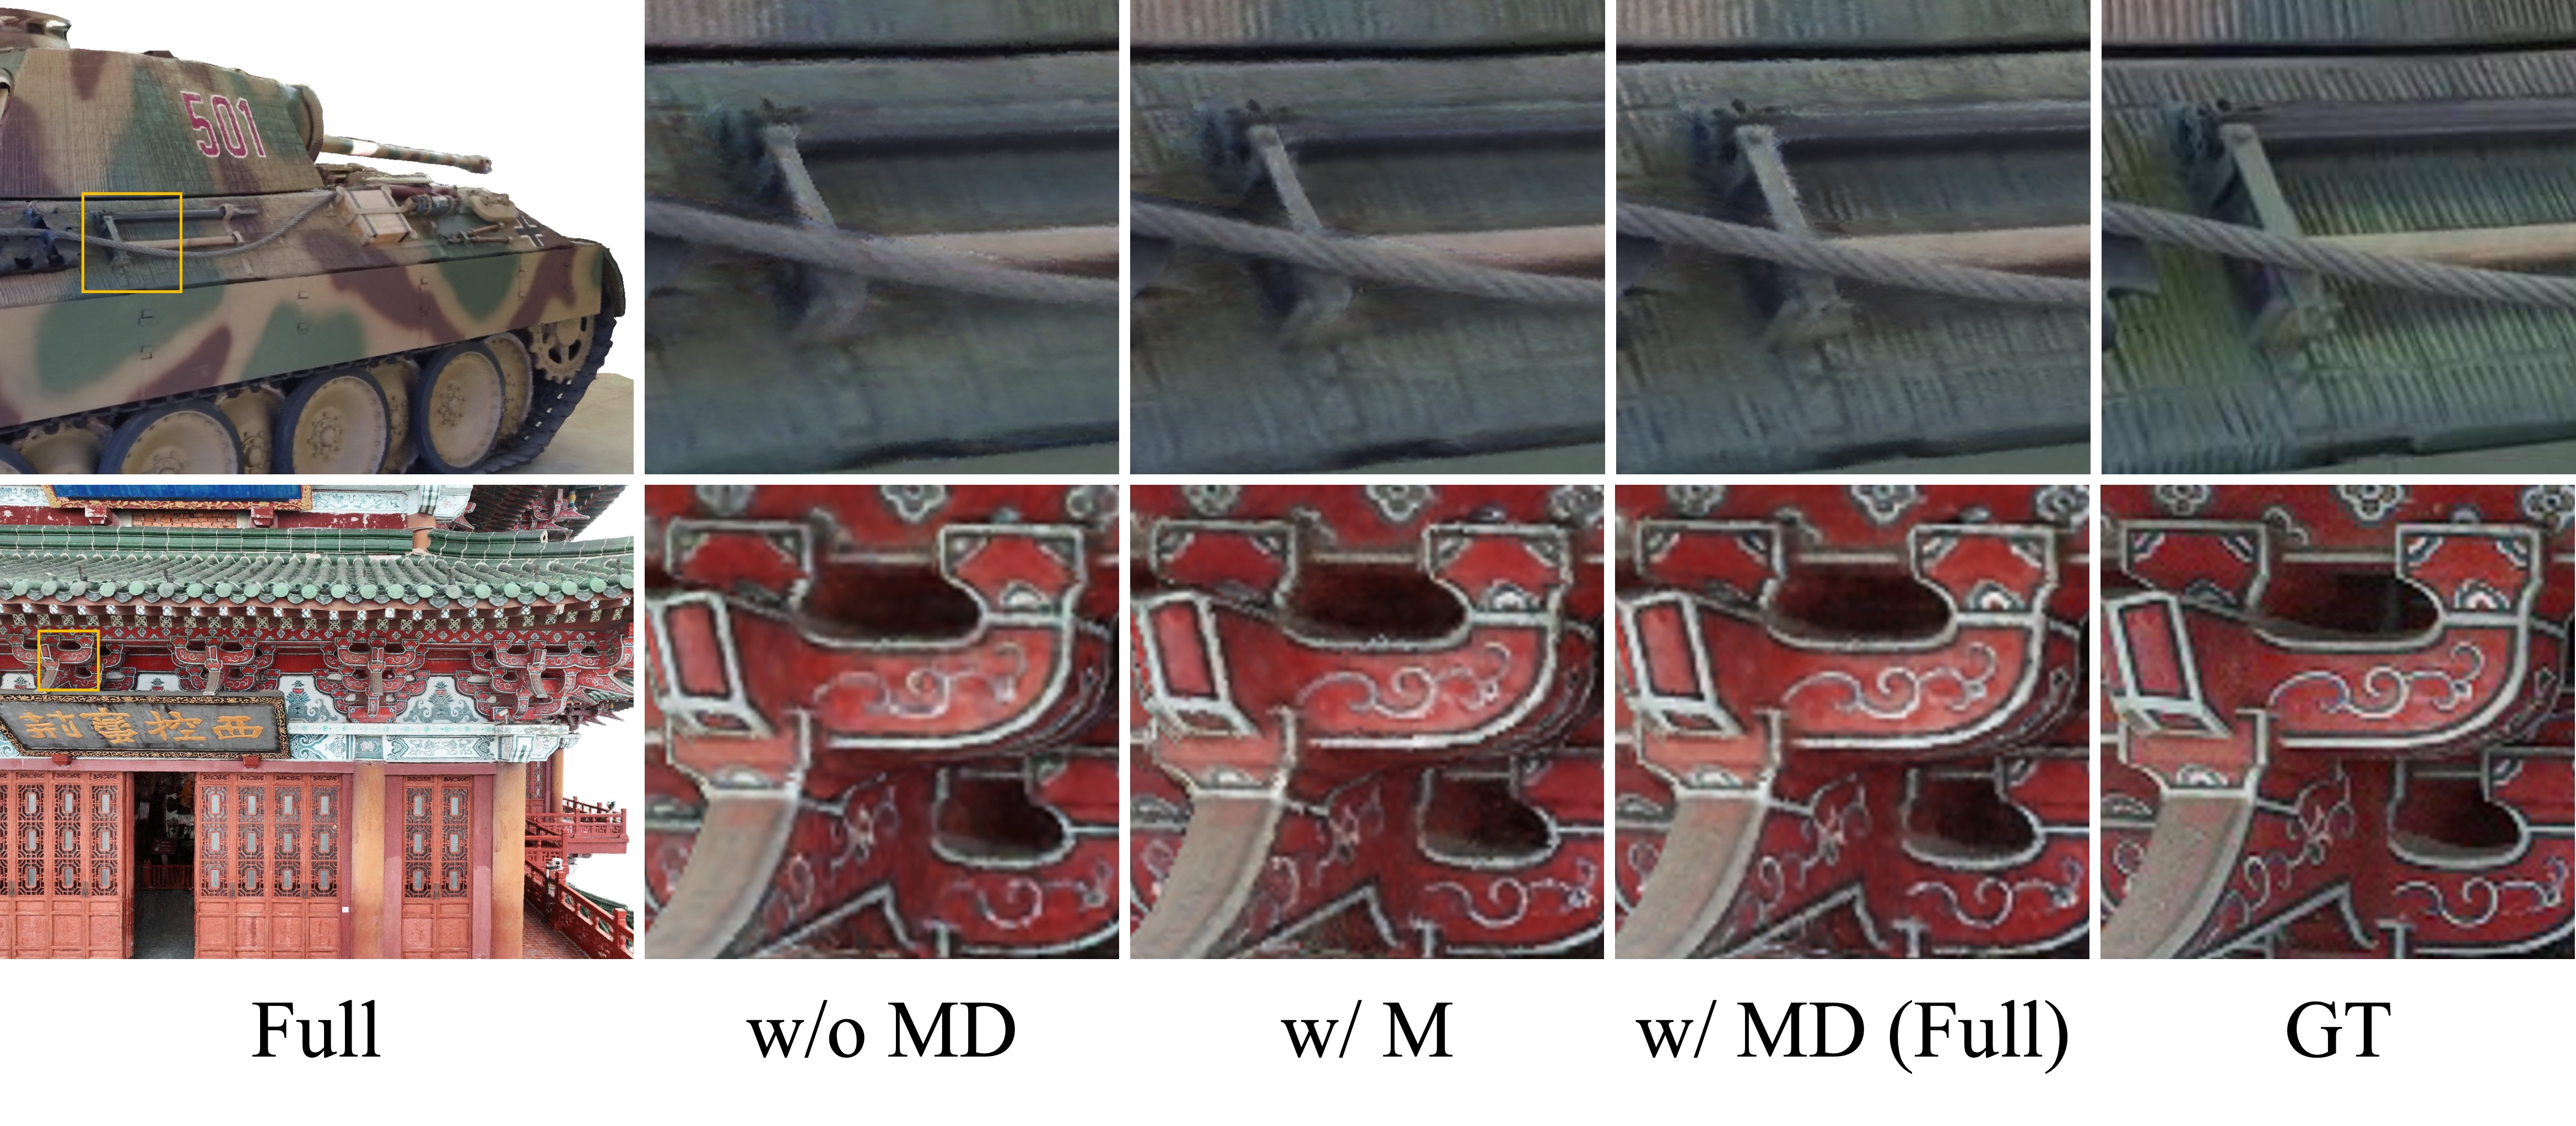}
    \vspace{-2.5em}
    \caption{Qualitative comparisons of novel view synthesis with different levels of featurization enhancements. Sharp details can be effectively recovered with surface multisampling (M) and manifold deformation (D).}
    \hfill
    \vspace{-1.0em}
    \label{fig:ablation_md}
\end{figure}
% \begin{table}[htbp]
% \scriptsize
% \setlength{\tabcolsep}{3.2mm}{
% \footnotesize
% \begin{tabular}{ccccc}
% \hline
% \multicolumn{1}{c}{\# Faces} & {Mem. of Mesh} & PSNR$\uparrow$ & SSIM$\uparrow$ & LPIPS$\downarrow$ \\ \hline
% 10M & {0.9GB} & {23.02} & {0.786} & {0.113} \\ 
% % 5M & {0.5GB} & {-} & {-} & {-} \\
% % 2M & {0.2GB} & {-} & {-} & {-} \\ 
% 1M & {90MB} & {22.84} & {0.782} & {0.114} \\
% % 0.1M & {9MB} & {20.72} & {0.674} & {0.196} \\
% \hline
% \end{tabular}
% }
% \vspace{-1em}
% \caption{Ablation on mesh resolution. Metrics are reported on TW-Pavilion (Day). }\label{tab:ablation_mesh}
% \end{table}

% \begin{table}[htbp]
% \scriptsize
% \setlength{\tabcolsep}{6.0mm}{
% \footnotesize
% \begin{tabular}{cccc}
% \hline
% \multicolumn{1}{c}{\# Faces} & PSNR$\uparrow$ & SSIM$\uparrow$ & LPIPS$\downarrow$ \\ \hline
% 10M & {23.02} & {0.786} & {0.113} \\ 
% % 5M & {-} & {-} & {-} \\
% % 2M & {-} & {-} & {-} \\ 
% 1M & {22.84} & {0.782} & {0.114} \\
% % 0.1M & {20.72} & {0.674} & {0.196} \\
% \hline
% \end{tabular}
% }
% \vspace{-1em}
% \caption{Ablation on mesh resolution. 
% % Metrics are reported on TW-Pavilion (Day). 
% }\label{tab:ablation_mesh}
% \end{table}

\begin{table}[htbp]
\scriptsize
\setlength{\tabcolsep}{1.3mm}{
\footnotesize
\begin{tabular}{ccccc}
\hline
\multicolumn{1}{c}{Method} & \#Primitives & PSNR$\uparrow$ & SSIM$\uparrow$ & LPIPS$\downarrow$ \\ \hline
Ours & 16M & {17.61} & {0.724} & {0.206} \\ 
Ours & 8M & {17.58} & {0.722} & {0.210} \\
Ours & 4M & {17.52} & {0.714} & {0.218} \\
Ours & 2M & {17.47} & {0.704} & {0.226} \\
Ours & 1.6M & {17.44} & {0.696} & {0.233} \\
Ours & 1M & {17.35} & {0.680} & {0.242} \\
Ours & 0.5M & {17.14} & {0.645} & {0.264} \\
% 0.1M & {20.72} & {0.674} & {0.196} \\
\hline
3D Gaussian Splatting~\cite{kerbl20233d} & 3M & {17.25} & {0.670} & {0.380} \\
\hline
\end{tabular}
}
\vspace{-1em}
\caption{Mesh resolution ablation on the Sandie Spring scene.}
\label{tab:ablation_mesh_sandie}
\end{table}
\begin{table}[htbp]
\scriptsize
\setlength{\tabcolsep}{1.3mm}{
\footnotesize
\begin{tabular}{ccccc}
\hline
\multicolumn{1}{c}{Method} & \#Primitives & PSNR$\uparrow$ & SSIM$\uparrow$ & LPIPS$\downarrow$ \\ \hline
Ours & 10M & {23.02} & {0.786} & {0.113} \\ 
Ours & 5M & {22.94} & {0.785} & {0.112} \\
Ours & 2M & {22.87} & {0.783} & {0.112} \\ 
Ours & 1M & {22.84} & {0.782} & {0.114} \\
Ours & 0.5M & {22.44} & {0.767} & {0.125} \\
Ours & 0.2M & {22.07} & {0.749} & {0.140} \\
% 0.1M & {20.72} & {0.674} & {0.196} \\
\hline
3D Gaussian Splatting~\cite{kerbl20233d} & 3M & {21.52} & {0.752} & {0.225} \\
\hline
\end{tabular}
}
\vspace{-1.0em}
\caption{Mesh resolution ablation on the TW-Pavilion (Day) scene.}
\vspace{-1.0em}
\label{tab:ablation_mesh_twg}
\end{table}

\par\noindent\textbf{Mesh Resolution.} 
% \guangyu{More scenes from GigaNVS and also Panther from Tanks\&Temples}
% \guangyu{A Curve where the x-axis is the resol. to indicate our robustness and incapacity at the inflection point. }
We now present further demonstrations regarding the robustness of our representation w.r.t. the input mesh resolution. The ablations are performed on two challenging scenes (Sandie Spring and TW-Pavilion (Day)) from the \texttt{GigaNVS} dataset. The quantitative evaluations on the two scenes are reported in Table~\ref{tab:ablation_mesh_sandie} and Table~\ref{tab:ablation_mesh_twg} respectively, where \#Primitives denote the amount of triangle facets of our input mesh or the amount of gaussians used in \cite{kerbl20233d}, and `M' denotes a million. Remarkably, our representation shows strong robustness w.r.t. the mesh resolution and outperforms 3DGS~\cite{kerbl20233d} with much lower discretization resolution. Unlike \cite{kerbl20233d}, our hash featurized manifold is essentially a neural-based representation which does not explicitly store per-primitive feature descriptors (and also the gradients during optimization), potentially being expressive enough independent of the discretization resolution. On the other hand, our method can leverage a higher resolution mesh in a memory efficient way, where the mesh resolution only affects the memory for rasterization. For example, when rendering a 1K image, 3DGS~\cite{kerbl20233d} consumes 18G memory with 3 million gaussians, whereas our method only takes up 15G memory using a mesh with 10 million facets.

% \par\noindent\textbf{The Finest Resolution of Hash Encoding.}
% % \guangyu{a curve with both 1K and 5K, and qualitative comparisons on 1K and 5K.}
% The finest resolution of the conceptually expressed feature grids in hash encoding slightly influences the performance of our representation, and we empirically set it according to the scene complexity, scale variation and also the imaging resolution. In Fig.XX, we show how our performance on the TW-Pavilion (Day) scene is influenced by different choices of the finest resolutions. The hash table size is fixed as 2$^{22}$ and the experiments are performed on both 1K resolution and 5K resolution. In Table XX, we summarize the finest resolutions used for different scenes from the \texttt{GigaNVS} dataset.
% % \par\noindent\textbf{Film Conditioning.}

\section{Necessity for Improving Feature Resolution}
% Potentially move the following discussions to supplementary. 
\begin{figure}[htb]
    %\centering
    %\centering
    
    \newcommand{\figw}{0.45} % can bigger than 1
    %\begin{minipage}{\colw\linewidth}
    \vspace{-1em}
    \centering
    \includegraphics[width=\figw\textwidth,trim={0cm 0cm 0cm 0cm},clip]{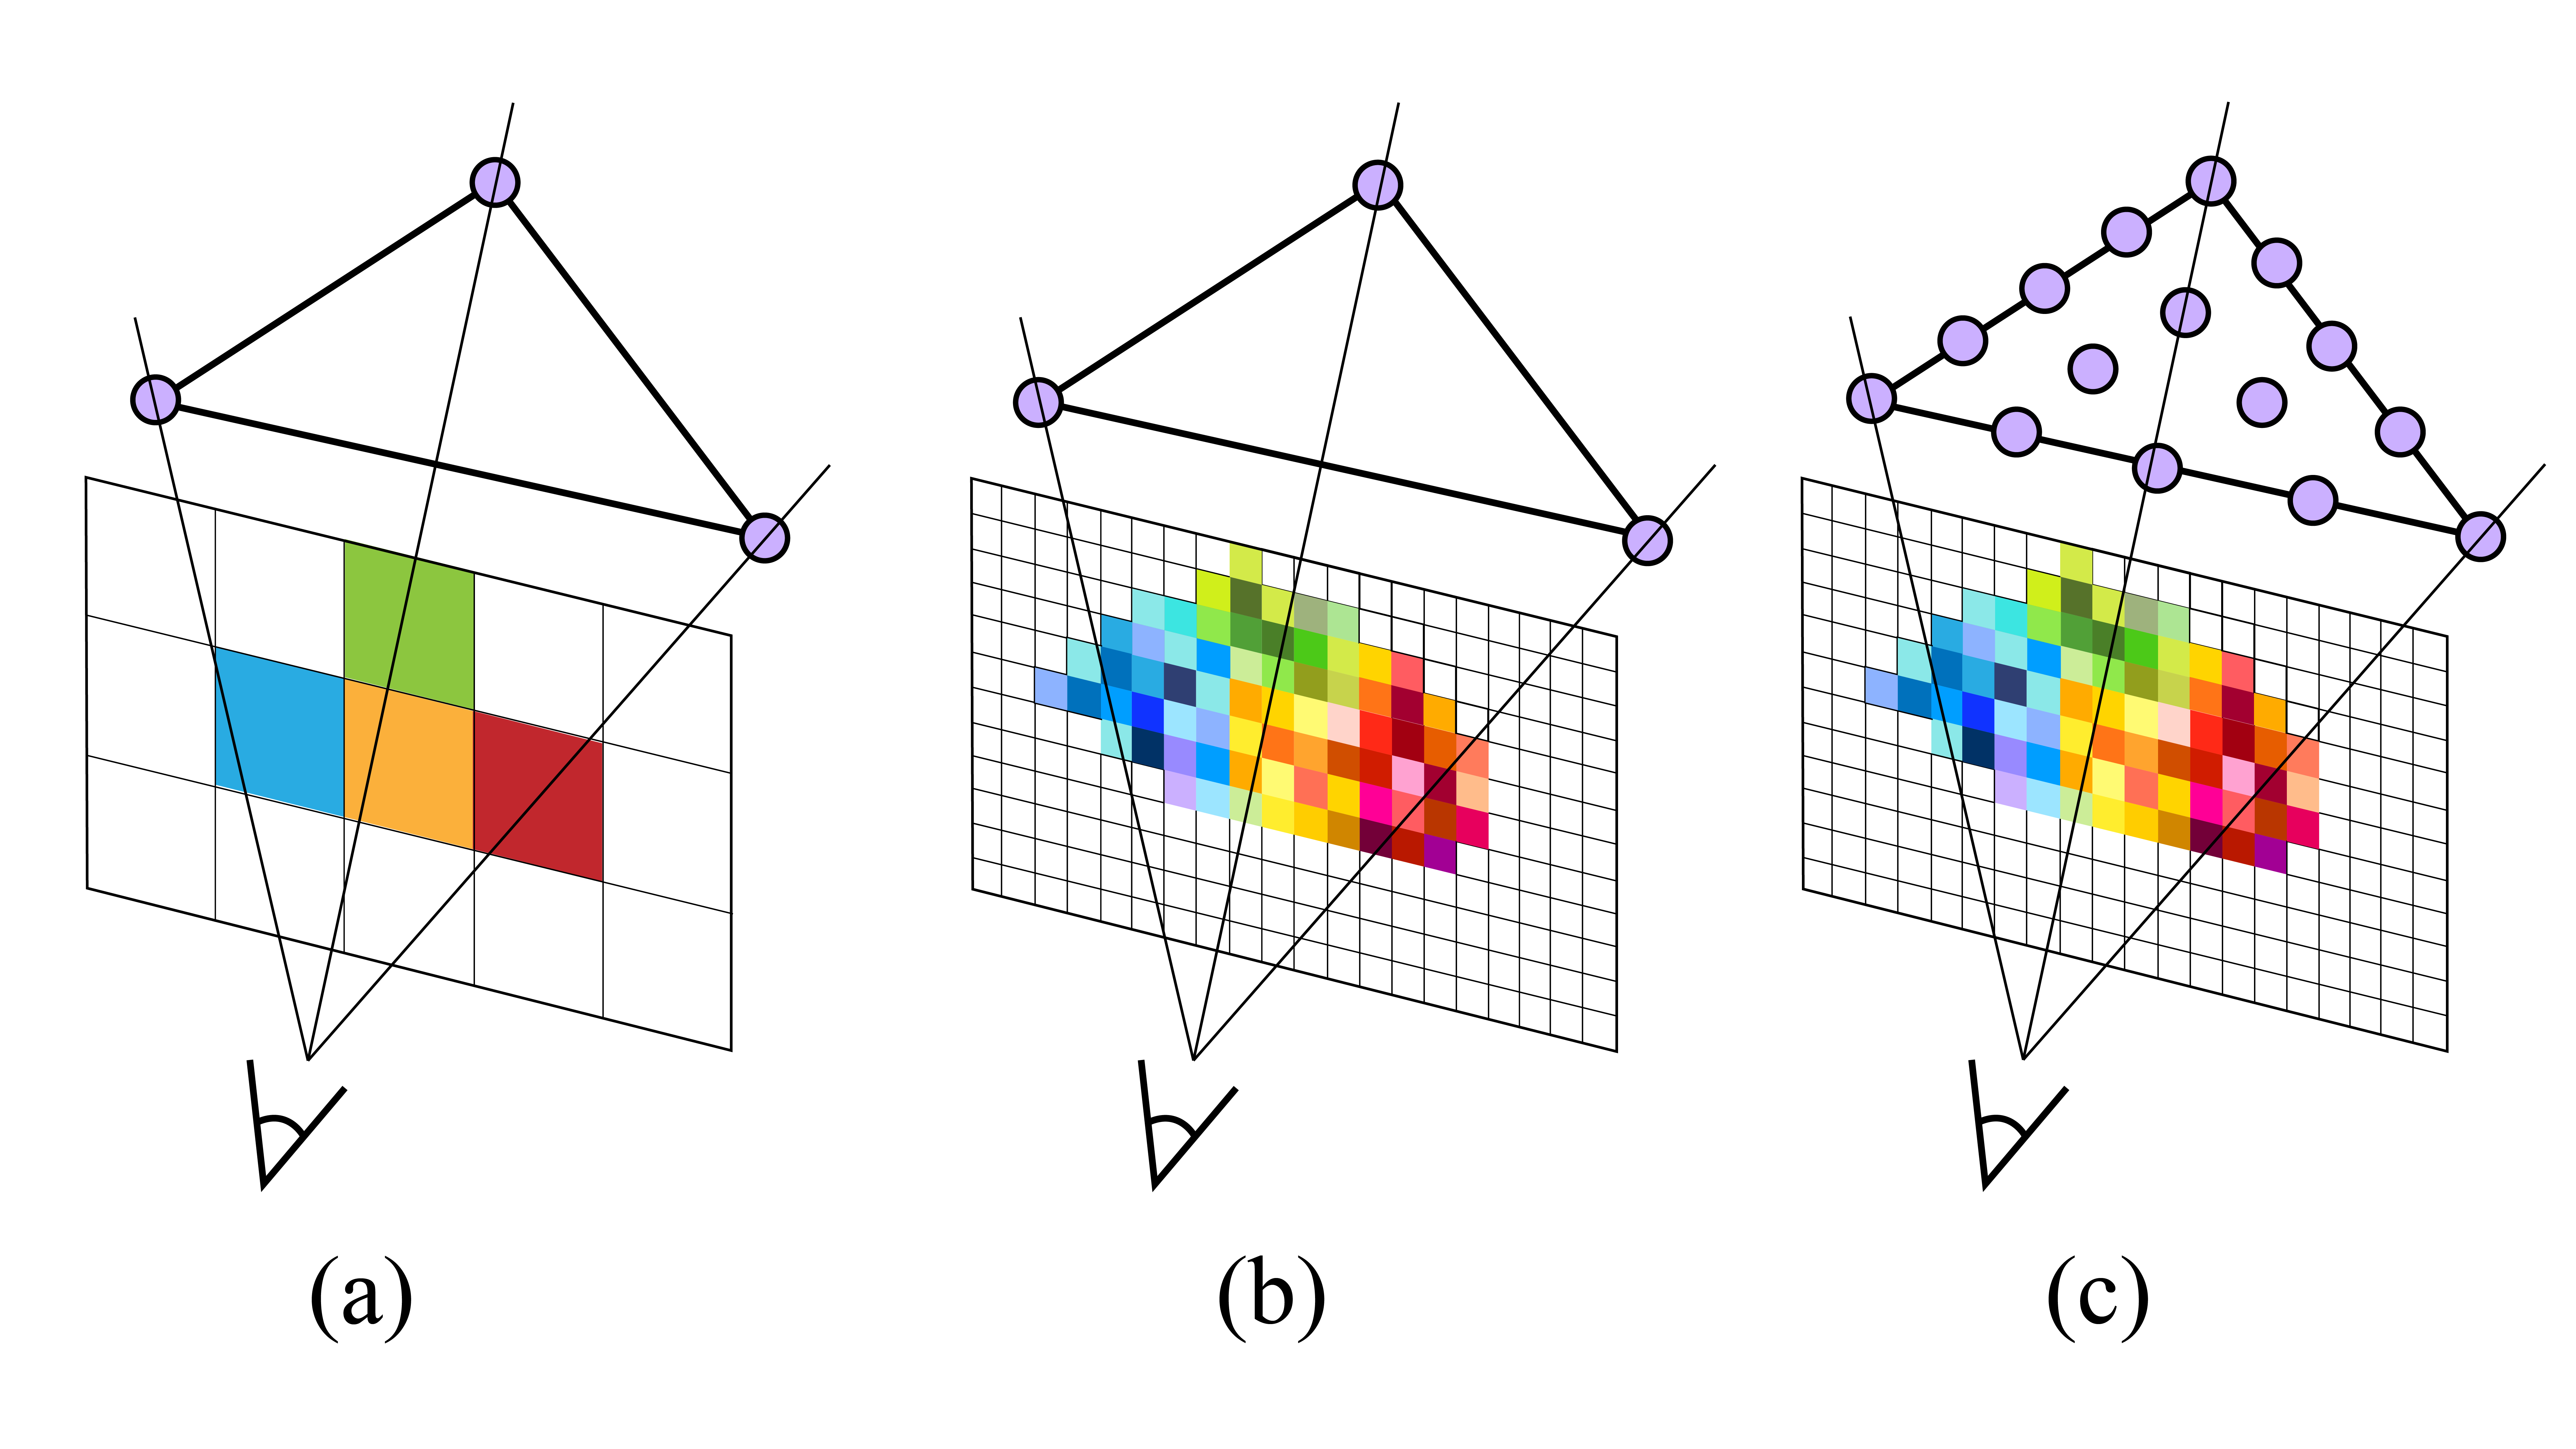}
    \vspace{-1em}
    \caption{Illustration of the featuremetric resolution issue. }
    \hfill
    \vspace{-1em}
    \label{fig:feat_resol}
\end{figure}
\begin{figure*}[htb]
    %\centering
    %\centering
    
    \newcommand{\figw}{1.0} % can bigger than 1
    %\begin{minipage}{\colw\linewidth}
    % \vspace{-1em}
    \centering
    \includegraphics[width=\figw\textwidth,trim={0cm 0cm 0cm 0cm},clip]{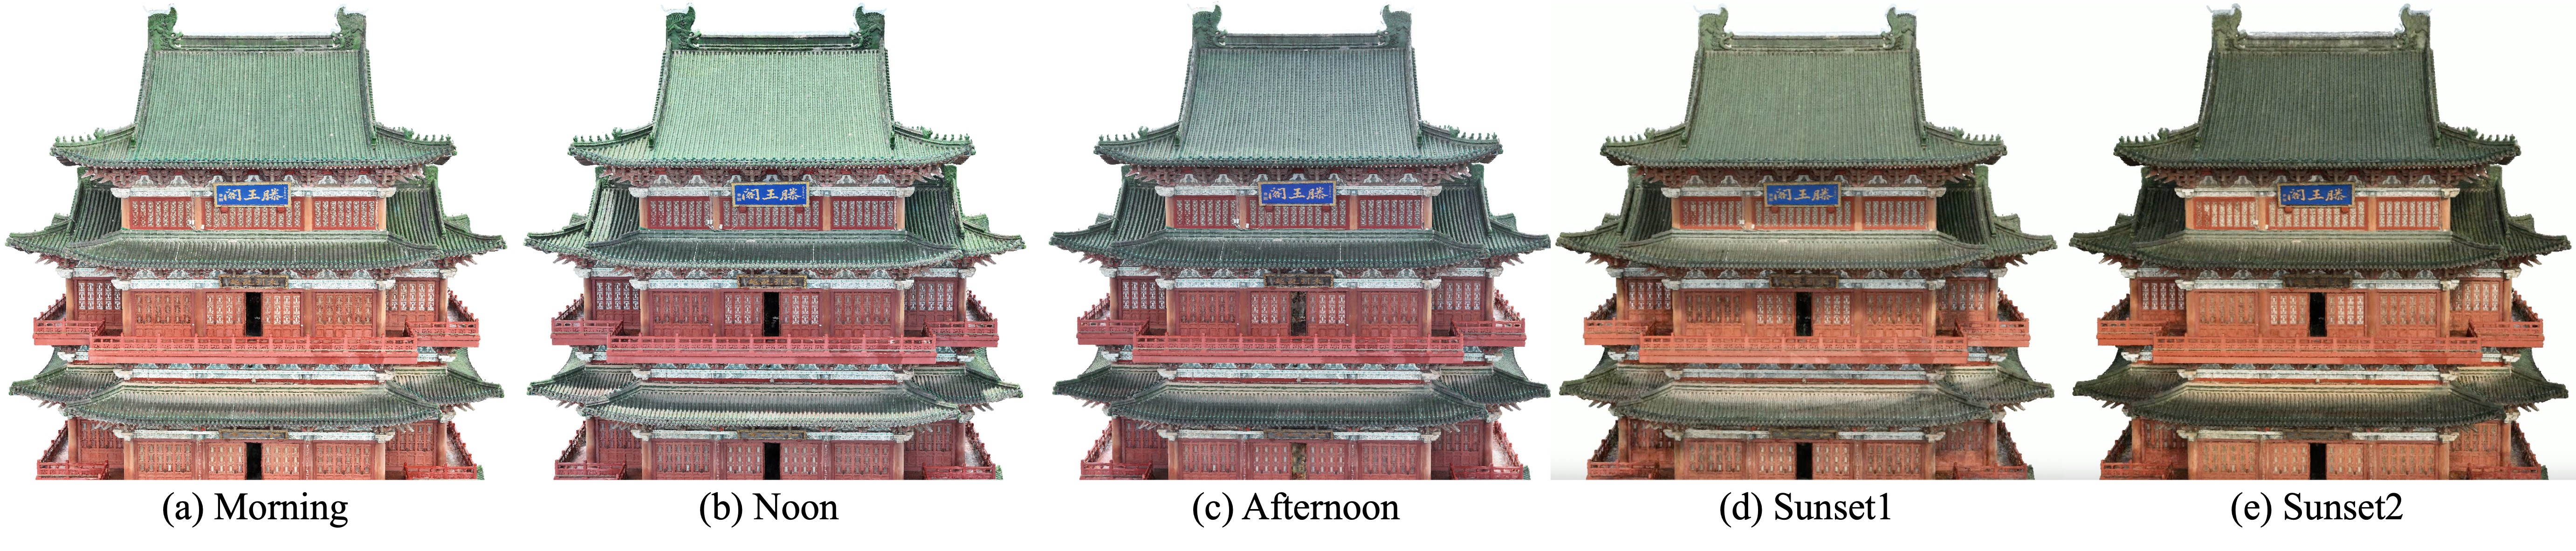}
    \vspace{-2.0em}
    \caption{Qualitative relighting results on the TW-Pavilion (Day) scene when varying the lighting embedding.}
    \hfill
    \vspace{-1.5em}
    \label{fig:qualitative_relit}
\end{figure*}
\begin{figure}[htb]
    %\centering
    %\centering
    
    \newcommand{\figw}{0.48} % can bigger than 1
    %\begin{minipage}{\colw\linewidth}
    % \vspace{-1em}
    \centering
    \includegraphics[width=\figw\textwidth,trim={0cm 0cm 0cm 0cm},clip]{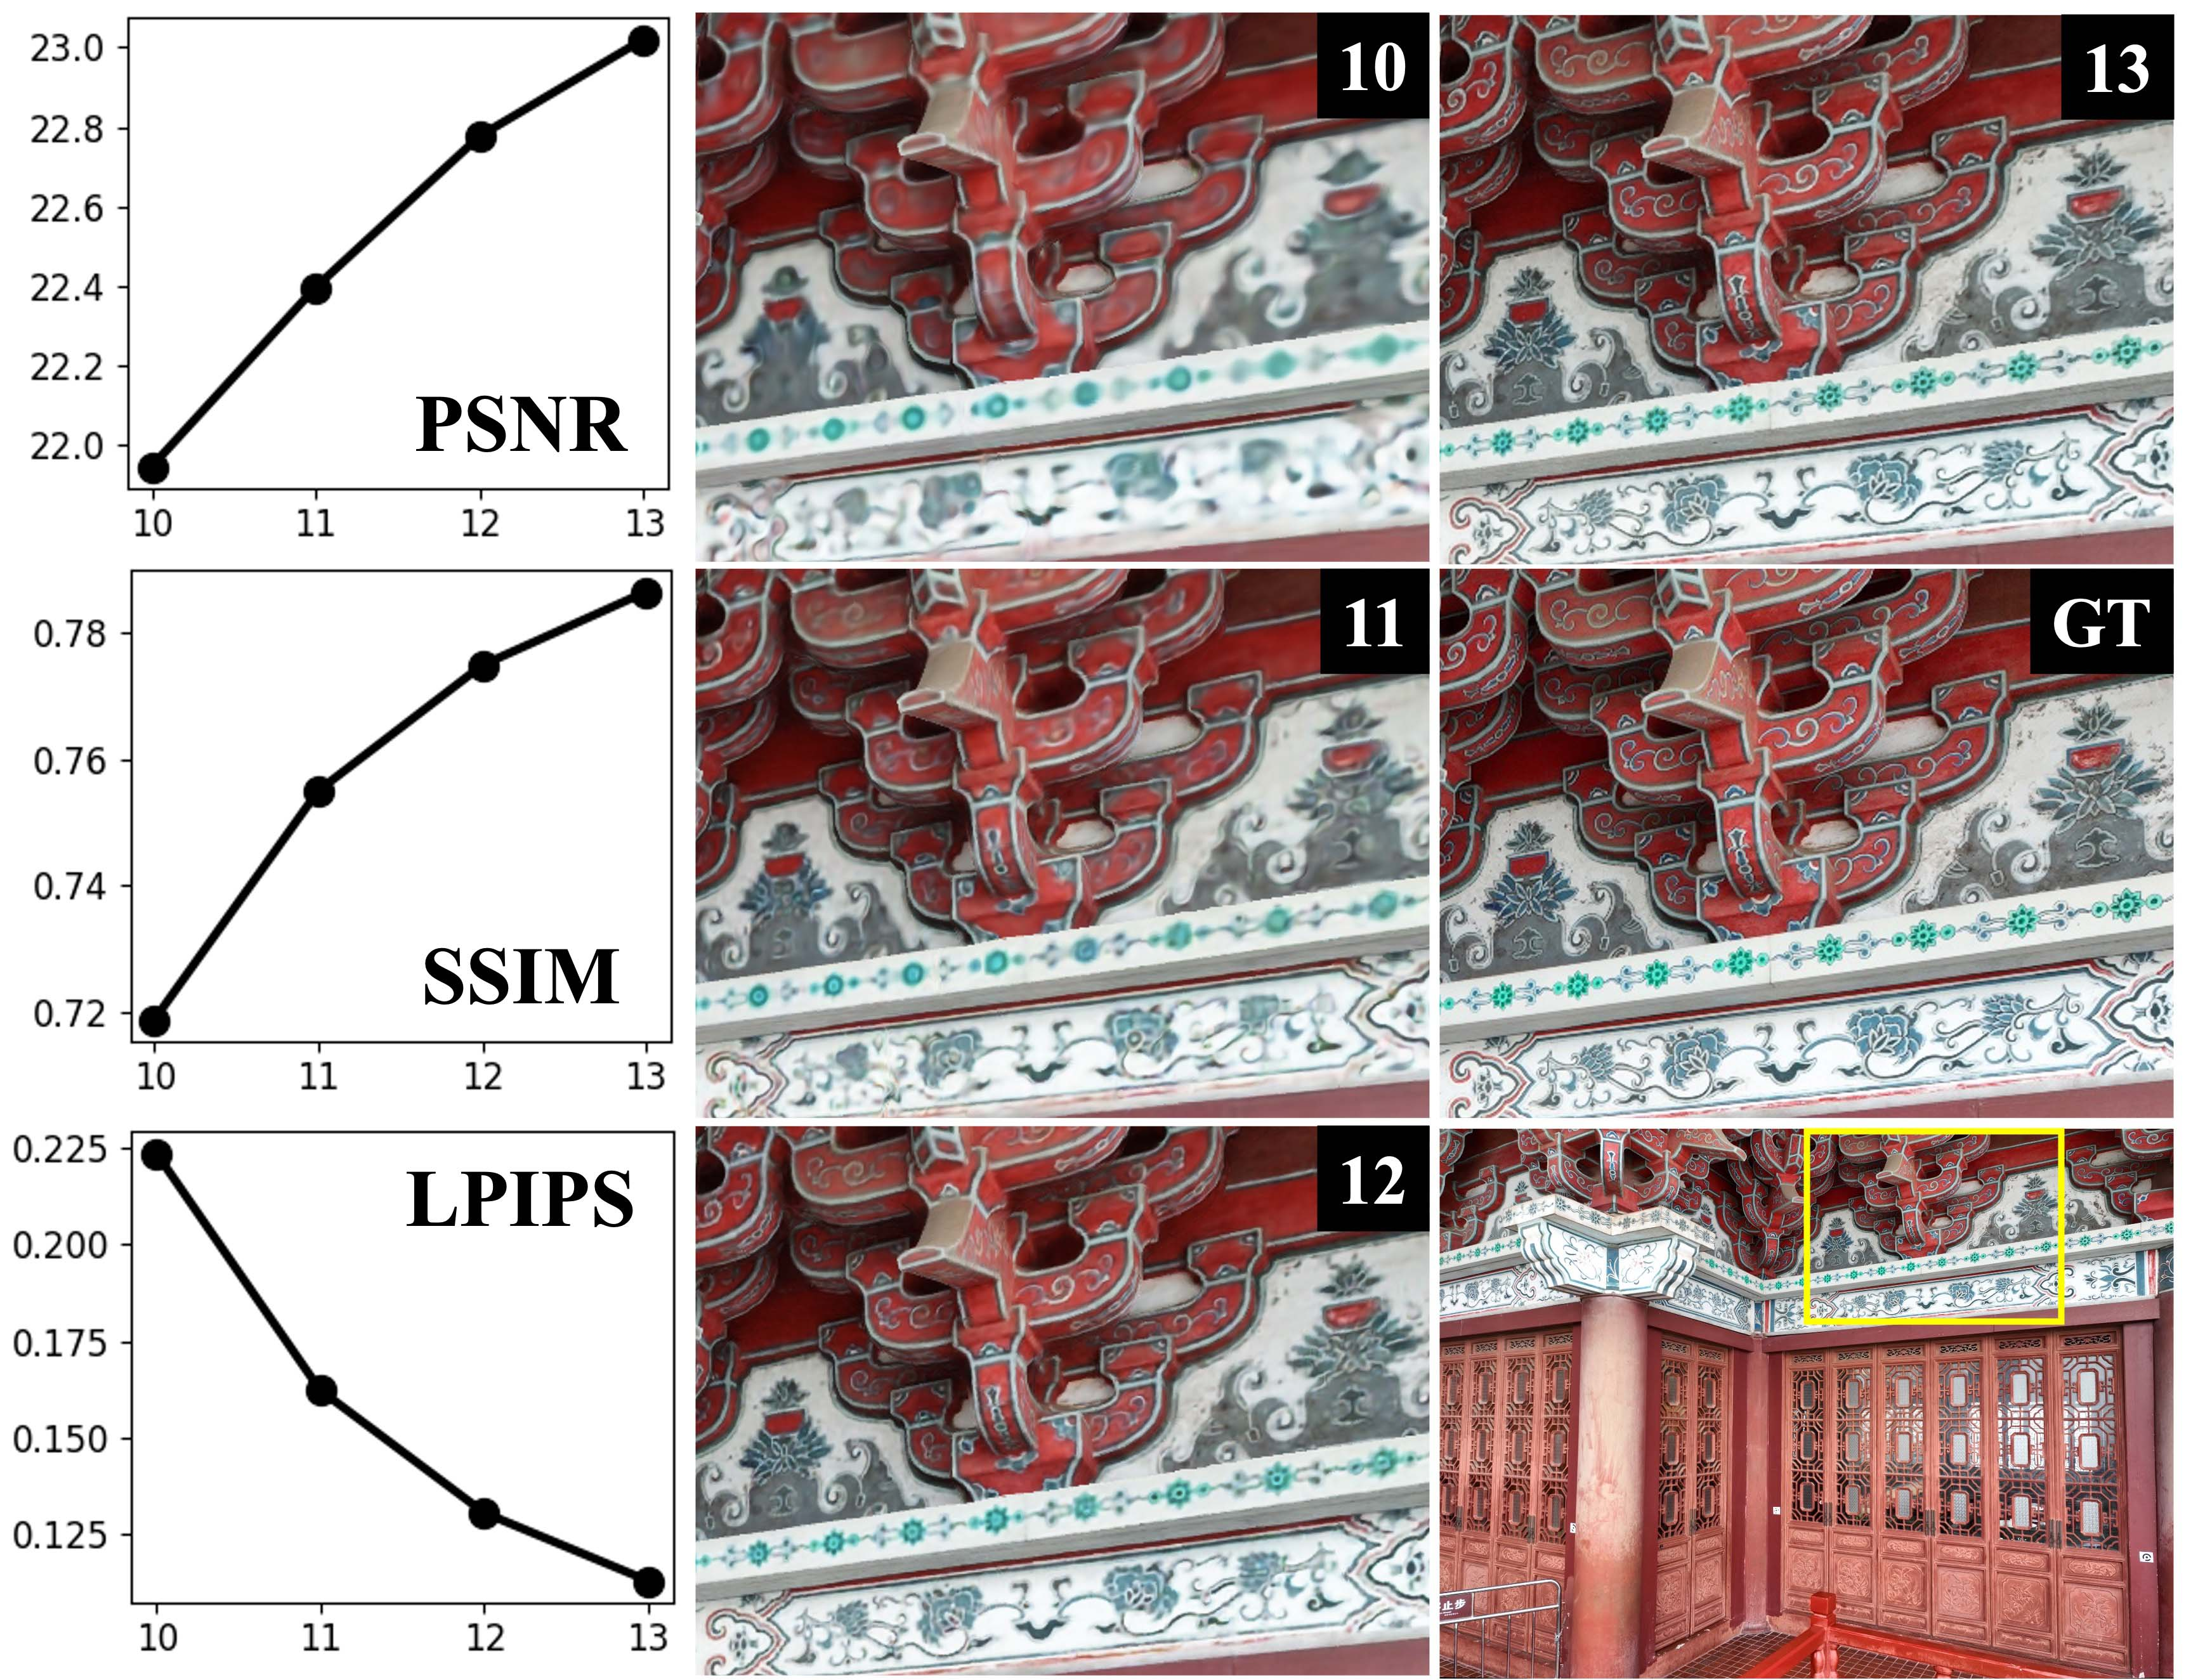}
    \vspace{-1.5em}
    \caption{Quantitative and qualitative evaluations with different featuremetric resolutions (2$^{10}$ $\sim$ 2$^{13}$).}
    \hfill
    \vspace{-2.2em}
    \label{fig:qualitative_resol}
\end{figure}

In contrast to early neural representations~\cite{mildenhall2021nerf, wang2021neus} that use a large global MLP to encode the entire scene, recent works~\cite{sun2022direct, muller2022instant, li2023neuralangelo, chen2022tensorf} tend to use a hybrid representation, i.e., a combination of the explicit volumetric featurization with a light-weight MLP decoder. In this way, the representational power can be effectively shifted from the MLP to local spatial features, which enables superior reconstruction quality and efficiency. 

In light of this, we hold that the spatial resolution of the underlying local features is strongly correlated to the expressivity of the representation, and it is essential to allocate local features with a sufficient resolution according to the scene complexity, scale variation, and the image resolution. We now give an intuitive illustration of this observation in Fig.~\ref{fig:feat_resol}. Assuming we have a coarse mesh with per-vertex learnable features, and we first consider small-scale simple scenes which are often captured at a medium distance with relatively low-resolution. As shown in Fig.~\ref{fig:feat_resol}~(a), a single surface primitive, i.e., a triangle facet in this case, only contains the information of very few pixels on the captured image. In this case, it is easy to accurately express the information of the pixels using the three feature descriptors at the vertices. However, for large-scale complex scenes with high-resolution or close-up captures, as illustrated in Fig.~\ref{fig:feat_resol}~(b), the pixel information covered by the same surface primitive is significantly enriched, making it difficult to fully describe the high-frequency pixel contents only by the vertex-defined features. In this case, the representation will produce blurry renderings. Note that representations based on other types of surface primitives like UV texels~\cite{10274871, thies2019deferred}, points~\cite{aliev2020neural, ruckert2022adop}, or Gaussians~\cite{kerbl20233d} also share the same intuition. Therefore, to tackle this issue, we should increase the featuremetric resolution to match the richness of pixels, which may significantly exceed the resolution of surface primitives, as shown in Fig.~\ref{fig:feat_resol}~(c). 

To verify the above intuition, we conduct ablations by varying the conceptually expressed finest resolution of hash encoding while keeping the hash table size fixed. The experiments are performed on the TW-Pavilion (Day) scene with 1K resolution. As shown in Fig.~\ref{fig:qualitative_resol}, increasing the finest resolution from 2$^{10}$ to 2$^{13}$ improves the quantitative metrics and enables more detailed view synthesis.  

\section{In-the-wild Relighting on \texttt{GigaNVS}}
Our method models the view-dependent colour $\boldsymbol{c} \in \mathbb{R}^3$ with an MLP-based implicit function $\mathcal{M}: \mathbb{R}^{LZ} \times \mathbb{R}^3 \mapsto \mathbb{R}^3$, which takes as inputs the queried hash feature $\mathcal{F}_{s}^{\mathcal{H}}(\boldsymbol{x}_s) \in \mathbb{R}^{LZ}$ and the view direction vector $\boldsymbol{d} \in \mathbb{R}^3$, i.e.,
\begin{equation}\label{eqn:vanilla_c}
    \boldsymbol{c} = \mathcal{M}(\mathcal{F}_{s}^{\mathcal{H}}(\boldsymbol{x}_s), \boldsymbol{d}).
\end{equation}

We can easily extend this formulation to implicitly account for the global illumination by introducing an additional lighting embedding $\boldsymbol{e}_{l}^{(k)} \in \mathbb{R}^{E}$: 
\begin{equation}\label{eqn:relit}
    \boldsymbol{c} = \mathcal{M}(\mathcal{F}_{s}^{\mathcal{H}}(\boldsymbol{x}_s), \boldsymbol{d}, \boldsymbol{e}_{l}^{(k)}).
\end{equation}

Specifically, we leverage the timestamps from the metadata to partition the collected imagery into $K$ subsets, where each subset has a very different illumination, and images within a subset share nearly the same illumination condition. We then assign a learnable lighting embedding $\boldsymbol{e}_{l}^{(\cdot)}$ for each subset, and so we have $K$ lighting embeddings $\{\boldsymbol{e}_{l}^{(k)}\}_{k=1}^{K}$ in total, representing $K$ different scene illuminations. Given a specific training view from the $k$-th subset, we only back-propagate the gradients to the related lighting embedding $\boldsymbol{e}_{l}^{(k)}$ during training. In this way, we can relight the rendering by varying the lighting embedding passed to the implicit function $\mathcal{M}$, and unseen illuminations can be synthesized by interpolating between an arbitrary pair of the latent embeddings:
\begin{equation}\label{eqn:relit_interp}
    \boldsymbol{e}_{l}^{(i, j, \tau)} = \tau \boldsymbol{e}_{l}^{(i)} + (1 - \tau) \boldsymbol{e}_{l}^{(j)},
\end{equation}
where $\tau \in [0, 1)$ is a scalar value denoting the interpolation weight. 

In Fig.~\ref{fig:qualitative_relit}, we show our relighting results at a novel view point, where we empirically set the dimensionality of the lighting embeddings as $E=8$. The proposed lighting embedding effectively reasons about the global illumination effects and further improves the rendering fidelity of real-world large-scale scenes. Please refer to the supplementary video to see the smoothly interpolated illuminations. 

\section{Visualizations of Surface Ambiguity}
\begin{figure}[htb]
    %\centering
    %\centering
    
    \newcommand{\figw}{0.48} % can bigger than 1
    %\begin{minipage}{\colw\linewidth}
    \vspace{-0.5em}
    \centering
    \includegraphics[width=\figw\textwidth,trim={0cm 0cm 0cm 0cm},clip]{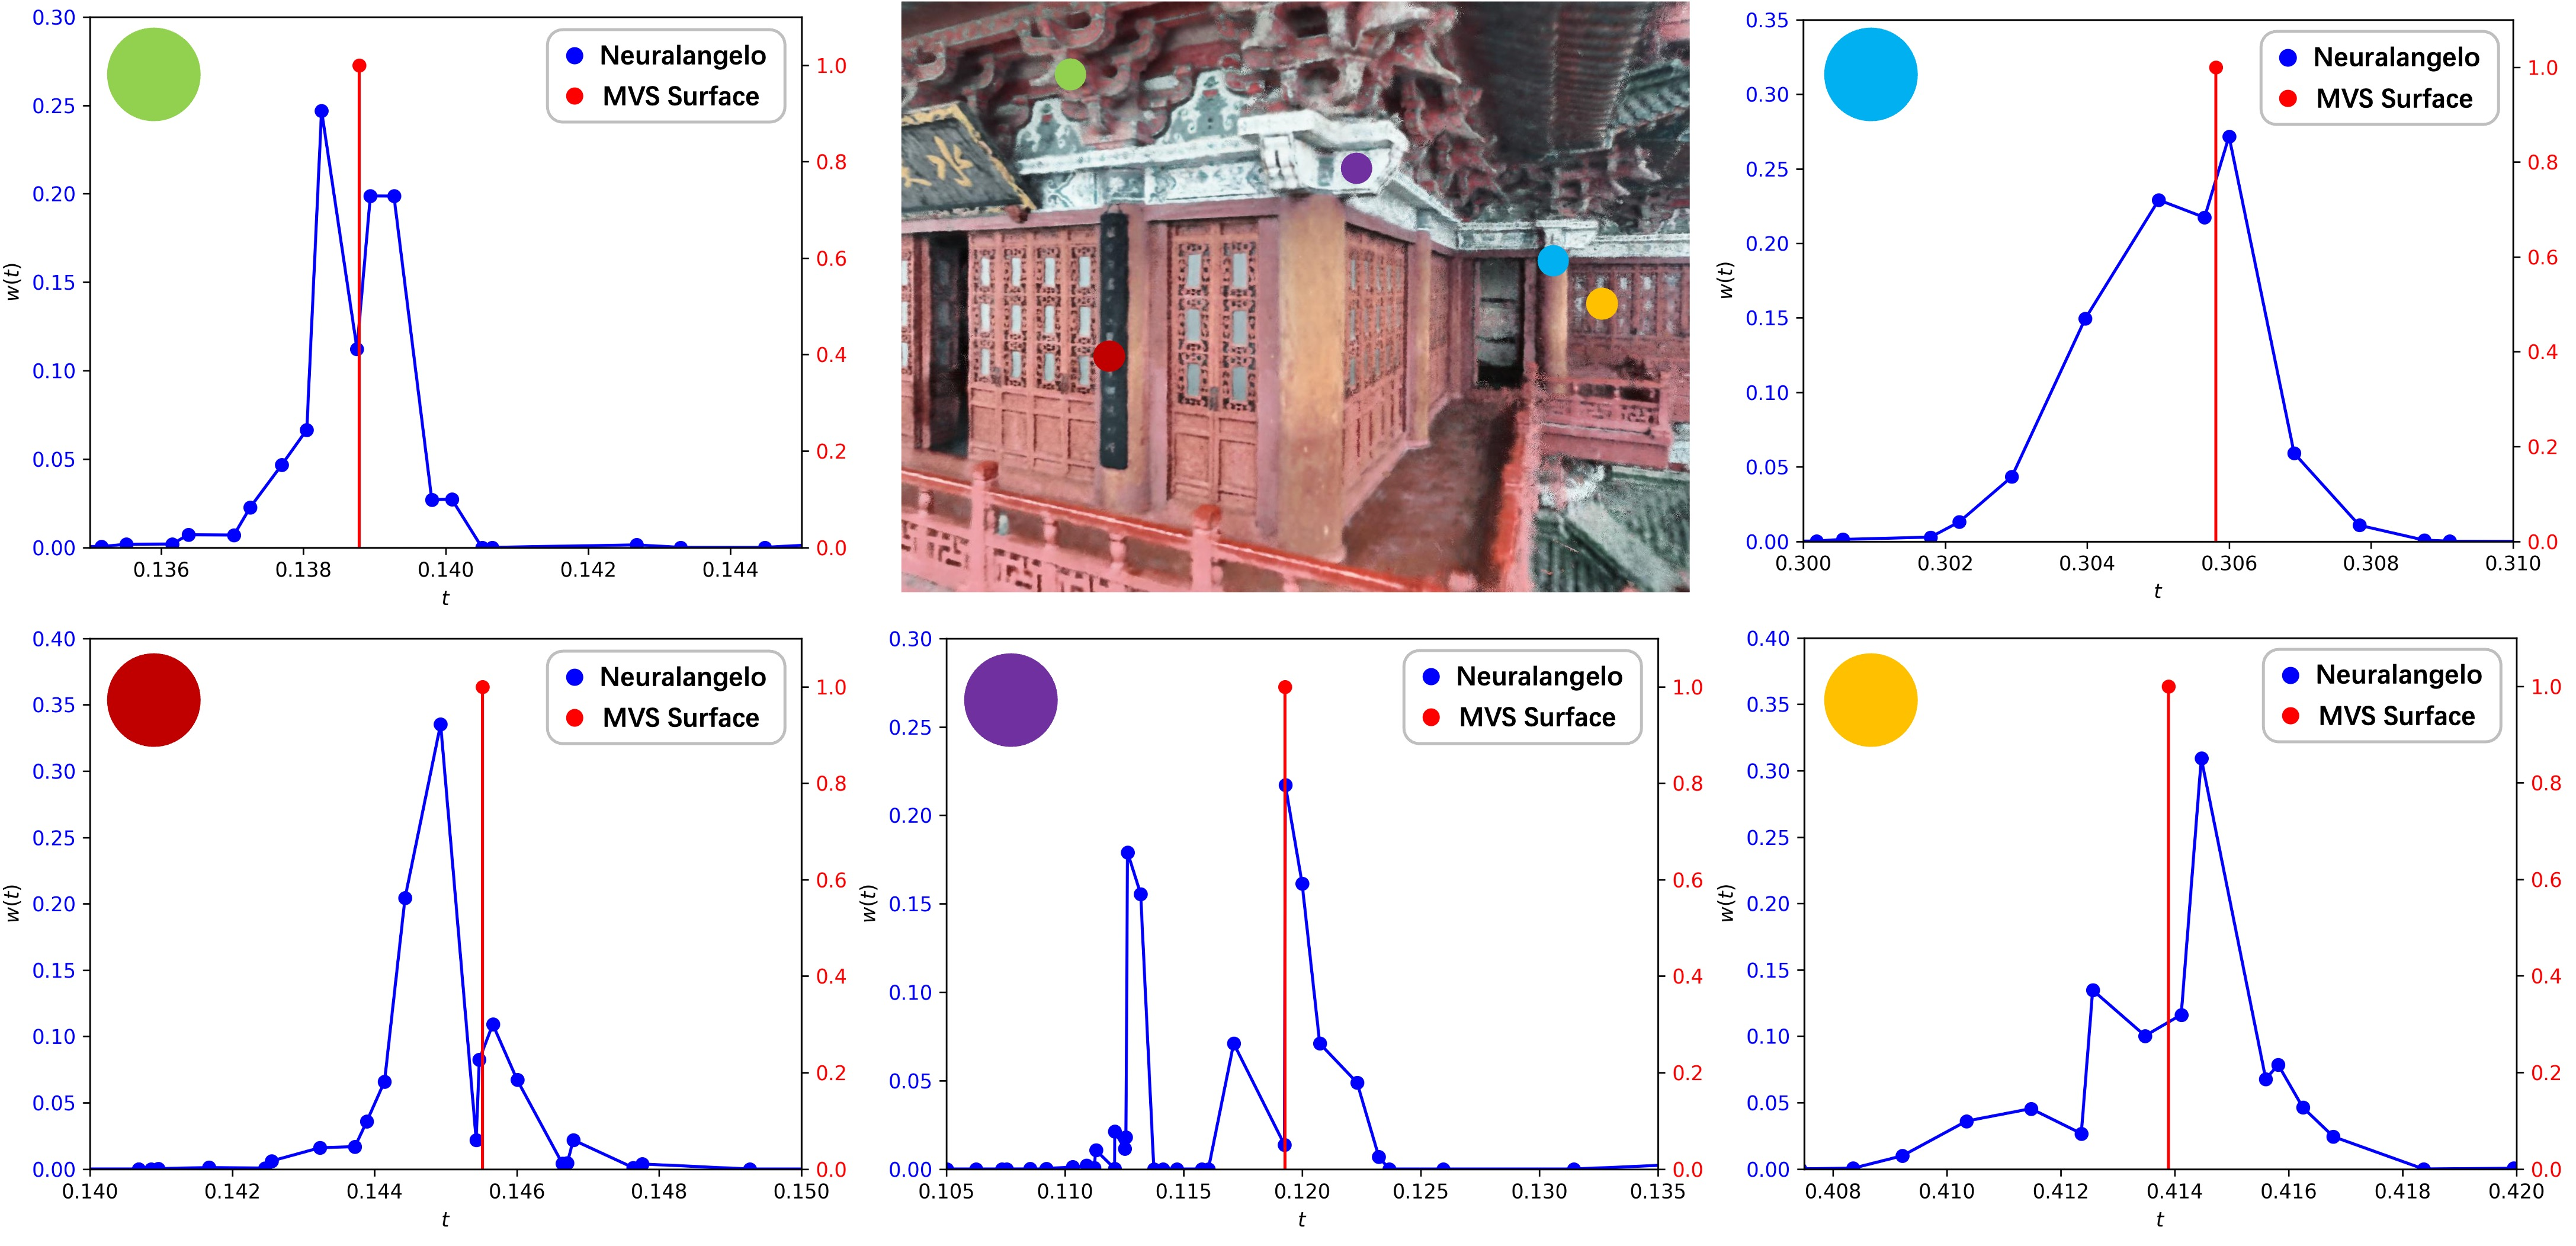}
    \vspace{-2em}
    \caption{Visualization of the volume rendering weight distributions of Neuralangelo~\cite{li2023neuralangelo}. The middle image is the final RGB rendering. In each surrounding sub-figure, we plot the weight $w(t)$ for each individual sample at certain normalized distance $t$ traced from one of the labeled pixels. The red vertical lines denote the surface locations calculated by mesh rasterization. For brevity, we only show important samples near the surface. 
    % and the horizontal axis $t$ denotes the normalized ray distance when the entire scene is transformed into a unit bounding sphere.
    }
    \hfill
    \vspace{-1em}
    \label{fig:vol_weight}
\end{figure}
In Fig.~\ref{fig:vol_weight}, we take Neuralangelo~\cite{li2023neuralangelo} as an example and visualize the weight distributions (the blue dot curves in the surrounding sub-figures) along the labeled pixel rays from the middle rendered image. Note that we use the mesh surface (the red vertical lines) reconstructed from MVS to densely supervise the SDF field in 3D~\cite{fu2022geo} throughout the experiments. However, the resulting weight distributions still scatter across a thick region, where most samples are in lack of multi-view consistency yet assigned with high volume rendering weight. As a result, these non-surface samples induce colour ambiguity and propagate inconsistent colour gradients to the surface sample, thus leading to excessive blurries that can be found in the rendering. 

\section{Limitations and Future Work}
Given that our representation is essentially a surface-based featurization, the incompleteness of the mesh reconstruction (e.g., far-away background regions or the holes caused by erroneous correspondence) is inevitably reflected in the rendering. However, since our primary focus is real-world large-scale scene reconstruction, where highly-specular surfaces or large textureless regions are not commonly witnessed, the mesh reconstructed by existing MVS methods is generally reliable enough. Regarding the background issue, we can easily address it by incorporating another volumetric neural field, similar to \cite{barron2023zip, barron2022mip, li2023neuralangelo}. Except for the incompleteness, remarkably, our method is robust to other topological or geometric degradations without the need to explicitly fix the mesh $-$ see the `$\leq$1M' results in Fig.~\ref{fig:qualitative_mesh} and~\ref{fig:qualitative_mesh_twg}, where our method effectively represents the missing details of the suboptimal geometry. 
% The reason is that both multi-resolution encoding and manifold deformation offer robustness in querying multi-view consistent signals.

Our future work is to explore scalable differentiable rendering pipelines for more flexible optimization of the topology, and to investigate physically-based inverse rendering techniques for the explicit acquisition of the underlying intrinsic properties, which is indispensable for downstream industrial applications. \\
