# Supplementary material for: XScale-NVS: Cross-Scale Novel View Synthesis with Hash Featurized Manifold
Source: arXiv:2403.19517 source file (2024-03-28)
Supplement: Supplementary file 2 [file qualitative_supp.tex]

\begin{figure*}[htbp]
    \centering
    
    \newcommand{\figw}{1.0} % can bigger than 1
    \includegraphics[width=\figw\textwidth,trim={0cm 0cm 0cm 0cm},clip]{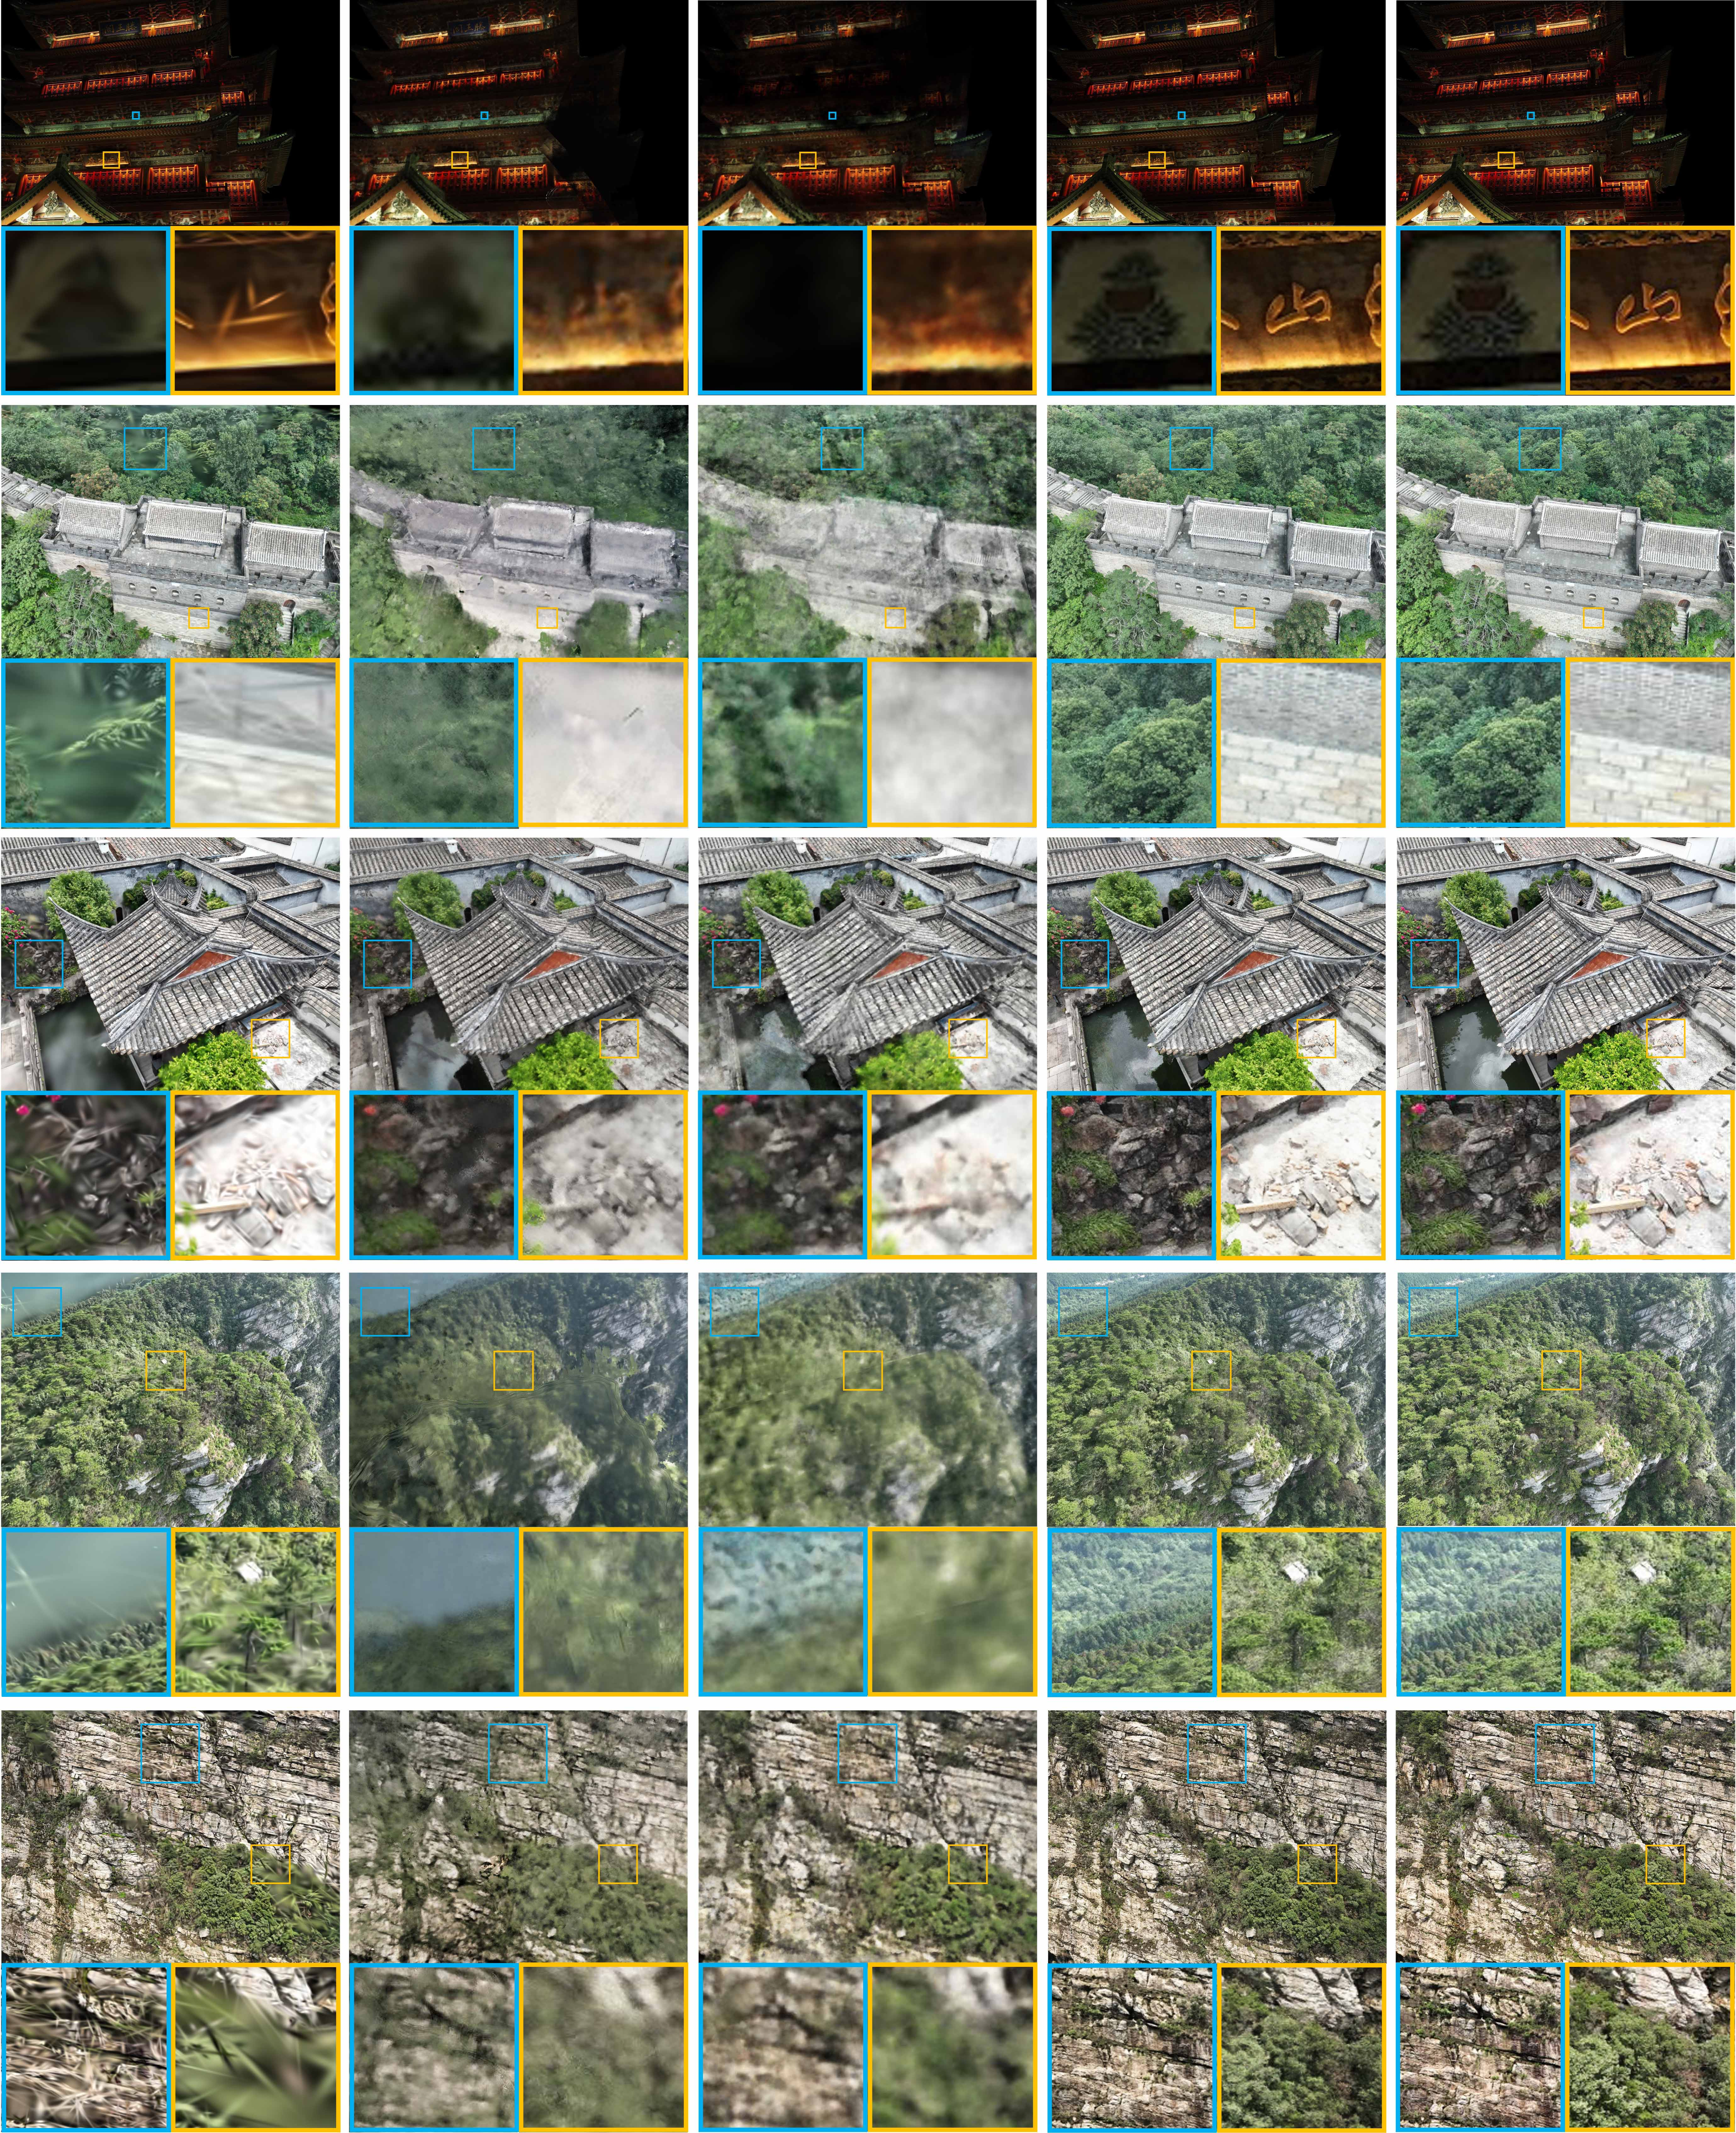}
\hfill
\vspace{-1.5em}
\centerline{\footnotesize{\hspace{-1.5em}
    (a) 3D Gaussian Splatting~\cite{kerbl20233d}\hspace{2.0em}(b) Neuralangelo~\cite{li2023neuralangelo}\hspace{5.0em}(c) iNGP~\cite{muller2022instant}\hspace{8.0em}(d) \textbf{Ours}\hspace{5.5em}
    (e) Ground Truth Image}}
\vspace{-1.5em}
\caption{Qualitative comparisons of 1K-resolution novel view synthesis on the \texttt{GigaNVS} dataset. Compared to \cite{muller2022instant, kerbl20233d, li2023neuralangelo}, our hash featurized manifold represents cross-scale contents with superior fidelity and effectively preserves the rich details of the original imagery.}
\label{fig:qualitative_supp}
\end{figure*}
