# Supplementary material for: XScale-NVS: Cross-Scale Novel View Synthesis with Hash Featurized Manifold
Source: arXiv:2403.19517 source file (2024-03-28)
Supplement: Supplementary file 3 [file tab_dataset_supp.tex]

\begin{table}[htbp]
\scriptsize
\setlength{\tabcolsep}{3.2mm}{
\footnotesize
\begin{tabular}{cccc}
\hline
{Scene} & Area ($m^2$) & \#Images & Resolution \\ \hline
TW-Pavilion (Day) & $1.3\times 10^4$ & 10,999 & 5K/8K \\ 
TW-Pavilion (Night) & $1.3\times 10^4$ & 1,687 & 5K/8K \\ 
Lanes \& Alleys & $4.5\times 10^5$ & 18,206 & 5K/8K \\ 
The Great Wall (T3) & $3\times 10^6$ & 7,441 & 5K/8K \\ 
The Great Wall (T2) & $2\times 10^6$ & 6,372 & 5K/8K \\ 
The Five Old Peaks & $1.5\times 10^6$ & 3,960 & 5K/8K \\ 
Sandie Spring & $3\times 10^6$ & 5,474 & 5K/8K \\ 
\hline
\end{tabular}
}
\vspace{-1em}
\caption{Statistics of the \texttt{GigaNVS} dataset.}\label{tab:dataset}
\vspace{-1em}
\end{table}
