# Supplementary material for: XScale-NVS: Cross-Scale Novel View Synthesis with Hash Featurized Manifold
Source: arXiv:2403.19517 source file (2024-03-28)
Supplement: Supplementary file 4 [file tab_mesh_supp.tex]

% \begin{table}[htbp]
% \scriptsize
% \setlength{\tabcolsep}{3.2mm}{
% \footnotesize
% \begin{tabular}{ccccc}
% \hline
% \multicolumn{1}{c}{\# Faces} & {Mem. of Mesh} & PSNR$\uparrow$ & SSIM$\uparrow$ & LPIPS$\downarrow$ \\ \hline
% 10M & {0.9GB} & {23.02} & {0.786} & {0.113} \\ 
% % 5M & {0.5GB} & {-} & {-} & {-} \\
% % 2M & {0.2GB} & {-} & {-} & {-} \\ 
% 1M & {90MB} & {22.84} & {0.782} & {0.114} \\
% % 0.1M & {9MB} & {20.72} & {0.674} & {0.196} \\
% \hline
% \end{tabular}
% }
% \vspace{-1em}
% \caption{Ablation on mesh resolution. Metrics are reported on TW-Pavilion (Day). }\label{tab:ablation_mesh}
% \end{table}

% \begin{table}[htbp]
% \scriptsize
% \setlength{\tabcolsep}{6.0mm}{
% \footnotesize
% \begin{tabular}{cccc}
% \hline
% \multicolumn{1}{c}{\# Faces} & PSNR$\uparrow$ & SSIM$\uparrow$ & LPIPS$\downarrow$ \\ \hline
% 10M & {23.02} & {0.786} & {0.113} \\ 
% % 5M & {-} & {-} & {-} \\
% % 2M & {-} & {-} & {-} \\ 
% 1M & {22.84} & {0.782} & {0.114} \\
% % 0.1M & {20.72} & {0.674} & {0.196} \\
% \hline
% \end{tabular}
% }
% \vspace{-1em}
% \caption{Ablation on mesh resolution. 
% % Metrics are reported on TW-Pavilion (Day). 
% }\label{tab:ablation_mesh}
% \end{table}

\begin{table}[htbp]
\scriptsize
\setlength{\tabcolsep}{1.3mm}{
\footnotesize
\begin{tabular}{ccccc}
\hline
\multicolumn{1}{c}{Method} & \#Primitives & PSNR$\uparrow$ & SSIM$\uparrow$ & LPIPS$\downarrow$ \\ \hline
Ours & 16M & {17.61} & {0.724} & {0.206} \\ 
Ours & 8M & {17.58} & {0.722} & {0.210} \\
Ours & 4M & {17.52} & {0.714} & {0.218} \\
Ours & 2M & {17.47} & {0.704} & {0.226} \\
Ours & 1.6M & {17.44} & {0.696} & {0.233} \\
Ours & 1M & {17.35} & {0.680} & {0.242} \\
Ours & 0.5M & {17.14} & {0.645} & {0.264} \\
% 0.1M & {20.72} & {0.674} & {0.196} \\
\hline
3D Gaussian Splatting~\cite{kerbl20233d} & 3M & {17.25} & {0.670} & {0.380} \\
\hline
\end{tabular}
}
\vspace{-1em}
\caption{Mesh resolution ablation on the Sandie Spring scene.}
\label{tab:ablation_mesh_sandie}
\end{table}
