# Supplementary material for: XScale-NVS: Cross-Scale Novel View Synthesis with Hash Featurized Manifold
Source: arXiv:2403.19517 source file (2024-03-28)
Supplement: Supplementary file 5 [file tab_mesh_supp_twg.tex]

\begin{table}[htbp]
\scriptsize
\setlength{\tabcolsep}{1.3mm}{
\footnotesize
\begin{tabular}{ccccc}
\hline
\multicolumn{1}{c}{Method} & \#Primitives & PSNR$\uparrow$ & SSIM$\uparrow$ & LPIPS$\downarrow$ \\ \hline
Ours & 10M & {23.02} & {0.786} & {0.113} \\ 
Ours & 5M & {22.94} & {0.785} & {0.112} \\
Ours & 2M & {22.87} & {0.783} & {0.112} \\ 
Ours & 1M & {22.84} & {0.782} & {0.114} \\
Ours & 0.5M & {22.44} & {0.767} & {0.125} \\
Ours & 0.2M & {22.07} & {0.749} & {0.140} \\
% 0.1M & {20.72} & {0.674} & {0.196} \\
\hline
3D Gaussian Splatting~\cite{kerbl20233d} & 3M & {21.52} & {0.752} & {0.225} \\
\hline
\end{tabular}
}
\vspace{-1.0em}
\caption{Mesh resolution ablation on the TW-Pavilion (Day) scene.}
\vspace{-1.0em}
\label{tab:ablation_mesh_twg}
\end{table}
